# Supplementary material for: DREAMS: Density Functional Theory Based Research Engine for Agentic Materials Simulation
Source: arXiv:2507.14267 source file (2026-08-11)
Supplement: Supplementary file 1 [file SI.tex]

%%%%%%%%%%%%%%%%%%%%%%%%%%%%%%%%%%%%%%%%%%%%%%%%%%%%%%%%%%%%%%%%%%%%%
%% This is a (brief) model paper using the achemso class
%% The document class accepts keyval options, which should include
%% the target journal and optionally the manuscript type. 
%%%%%%%%%%%%%%%%%%%%%%%%%%%%%%%%%%%%%%%%%%%%%%%%%%%%%%%%%%%%%%%%%%%%%
\documentclass[journal=acscentscie,manuscript=suppinfo]{achemso}

%%%%%%%%%%%%%%%%%%%%%%%%%%%%%%%%%%%%%%%%%%%%%%%%%%%%%%%%%%%%%%%%%%%%%
%% Place any additional packages needed here.  Only include packages
%% which are essential, to avoid problems later. Do NOT use any
%% packages which require e-TeX (for example etoolbox): the e-TeX
%% extensions are not currently available on the ACS conversion
%% servers.
%%%%%%%%%%%%%%%%%%%%%%%%%%%%%%%%%%%%%%%%%%%%%%%%%%%%%%%%%%%%%%%%%%%%%
\usepackage[version=3]{mhchem} % Formula subscripts using \ce{}
\usepackage[utf8]{inputenc}
\usepackage[T1]{fontenc}
\usepackage{listings}%
\usepackage{graphicx}%
\usepackage{threeparttable}
\usepackage{subcaption}
\captionsetup[subfigure]{position=top, singlelinecheck=false,justification=raggedright}
\usepackage{multirow}
\usepackage{booktabs}
\usepackage{adjustbox}
\usepackage[table]{xcolor}
\usepackage{tabularx}
\usepackage{helvet}
\usepackage{enumitem}
\usepackage{setspace}
\usepackage{hyperref}

\usepackage{fvextra}    % Extension of fancyvrb
\usepackage[utf8]{inputenc}
\usepackage{pdfpages}

% thin gray rules by default
\arrayrulecolor{black!50}
\setlength{\arrayrulewidth}{0.3pt}

% define a thick rule (for top, after header, bottom)
\newcommand{\thickhline}{\specialrule{1.2pt}{0pt}{0pt}}

% \captionsetup[lstlisting]{labelformat=empty}

% \lstset{
%   numbers=left,
%   alsoletter={\#},
%   moredelim=[is][\phantom]{@}{@},  % hide @...@ from output
%   escapeinside={(*@}{@*)}, % allows LaTeX inside listings
% }

% Define a custom Python style
\lstdefinestyle{mystyle}{
    language=,
    % backgroundcolor=\color{gray!10},   
    commentstyle=\color{green!50!black},
    keywordstyle=\color{blue!80!black}\bfseries,
    numberstyle=\tiny\color{gray},
    stringstyle=\color{orange!90!black},
    basicstyle=\ttfamily\footnotesize,
    breaklines=true,                 
    captionpos=b,                    
    keepspaces=true,                 
    numbers=left,                    
    numbersep=5pt,                  
    showspaces=false,                
    showstringspaces=false,
    showtabs=false,                  
    tabsize=4,
    frame=single,
    numberblanklines=false,  % prevents line numbers for blank lines
    moredelim=**[is][\phantom]{@}{@},
    rulecolor=\color{gray!40}
}

%%%%%%%%%%%%%%%%%%%%%%%%%%%%%%%%%%%%%%%%%%%%%%%%%%%%%%%%%%%%%%%%%%%%%
%% If issues arise when submitting your manuscript, you may want to
%% un-comment the next line.  This provides information on the
%% version of every file you have used.
%%%%%%%%%%%%%%%%%%%%%%%%%%%%%%%%%%%%%%%%%%%%%%%%%%%%%%%%%%%%%%%%%%%%%
%%\listfiles

%%%%%%%%%%%%%%%%%%%%%%%%%%%%%%%%%%%%%%%%%%%%%%%%%%%%%%%%%%%%%%%%%%%%%
%% Place any additional macros here.  Please use \newcommand* where
%% possible, and avoid layout-changing macros (which are not used
%% when typesetting).
%%%%%%%%%%%%%%%%%%%%%%%%%%%%%%%%%%%%%%%%%%%%%%%%%%%%%%%%%%%%%%%%%%%%%

%%%%%%%%%%%%%%%%%%%%%%%%%%%%%%%%%%%%%%%%%%%%%%%%%%%%%%%%%%%%%%%%%%%%%
%% Meta-data block
%% ---------------
%% Each author should be given as a separate \author command.
%%
%% Corresponding authors should have an e-mail given after the author
%% name as an \email command. Phone and fax numbers can be given
%% using \phone and \fax, respectively; this information is optional.
%%
%% The affiliation of authors is given after the authors; each
%% \affiliation command applies to all preceding authors not already
%% assigned an affiliation.
%%
%% The affiliation takes an option argument for the short name.  This
%% will typically be something like "University of Somewhere".
%%
%% The \altaffiliation macro should be used for new address, etc.
%% On the other hand, \alsoaffiliation is used on a per author basis
%% when authors are associated with multiple institutions.
%%%%%%%%%%%%%%%%%%%%%%%%%%%%%%%%%%%%%%%%%%%%%%%%%%%%%%%%%%%%%%%%%%%%%
\author{Ziqi Wang}
\affiliation[UMichME]{Mechanical Engineering, University of Michigan, Ann Arbor, Michigan, USA}

\author{Hongshuo Huang}
\affiliation[UMichME]{Mechanical Engineering, University of Michigan, Ann Arbor, Michigan, USA}

\author{Hancheng Zhao}
\affiliation[UMichME]{Mechanical Engineering, University of Michigan, Ann Arbor, Michigan, USA}

\author{Changwen Xu}
\affiliation[UMichME]{Mechanical Engineering, University of Michigan, Ann Arbor, Michigan, USA}

\author{Shang Zhu}
\affiliation[UMichME]{Department of Mechanical Engineering, University of Michigan, Ann Arbor, Michigan, USA}

\author{Jan Janssen}
\email{janssen@mpi-susmat.de}
\affiliation[MaxPlanck]{Max-Planck-Institute for Sustainable Materials, Materials Informatics, Düsseldorf, Germany}

\author{Venkatasubramanian Viswanathan}
\email{venkvis@umich.edu}
\affiliation[UMichME]{Mechanical Engineering, University of Michigan, Ann Arbor, Michigan, USA}
\alsoaffiliation[UMichAE]{Aerospace Engineering, University of Michigan, Ann Arbor, Michigan, USA}

%%%%%%%%%%%%%%%%%%%%%%%%%%%%%%%%%%%%%%%%%%%%%%%%%%%%%%%%%%%%%%%%%%%%%
%% The document title should be given as usual. Some journals require
%% a running title from the author: this should be supplied as an
%% optional argument to \title.
%%%%%%%%%%%%%%%%%%%%%%%%%%%%%%%%%%%%%%%%%%%%%%%%%%%%%%%%%%%%%%%%%%%%%
\title[DFT Based Research Engine]
  {DREAMS: Density Functional Theory Based Research Engine for Automated Materials Screening}

%%%%%%%%%%%%%%%%%%%%%%%%%%%%%%%%%%%%%%%%%%%%%%%%%%%%%%%%%%%%%%%%%%%%%
%% Some journals require a list of abbreviations or keywords to be
%% supplied. These should be set up here, and will be printed after
%% the title and author information, if needed.
%%%%%%%%%%%%%%%%%%%%%%%%%%%%%%%%%%%%%%%%%%%%%%%%%%%%%%%%%%%%%%%%%%%%%
% \abbreviations{IR,NMR,UV}
\keywords{Hierarchical agents, LLM, Dynamic planning, Density Functional Theory (DFT), Computational materials science, Surface chemistry}

%%%%%%%%%%%%%%%%%%%%%%%%%%%%%%%%%%%%%%%%%%%%%%%%%%%%%%%%%%%%%%%%%%%%%
%% The manuscript does not need to include \maketitle, which is
%% executed automatically.
%%%%%%%%%%%%%%%%%%%%%%%%%%%%%%%%%%%%%%%%%%%%%%%%%%%%%%%%%%%%%%%%%%%%%
\begin{document}

\break
\section{Plan generated for Sol27LC challenge}
\begin{spacing}{1}
\begin{enumerate}[itemsep=0pt, parsep=0pt, topsep=0pt, partopsep=0pt]
    \item Create initial structure of BCC Li with experimental lattice constant of 3.451~\AA
    \item Find appropriate pseudopotential for Li
    \item Write initial DFT script for BCC Li
    \item Generate convergence test input files for cutoff energy and k-points
    \item Add resource suggestions for convergence test jobs
    \item Submit convergence test jobs to HPC and monitor completion
    \item Determine optimal parameters from convergence test results
    \item Generate equation of state (EOS) calculation input files using optimal parameters
    \item Add resource suggestions for EOS calculation jobs
    \item Submit EOS calculation jobs to HPC and monitor completion
    \item Read output files to extract energy values
    \item Calculate equilibrium lattice constant from EOS data
    \item Compare calculated lattice constant with experimental value and report results
\end{enumerate}
\end{spacing}

\section*{Full Canvas History for Sol27LC Challenge}
\begin{figure}[H]
    \centering
    \includegraphics[width=0.9\linewidth]{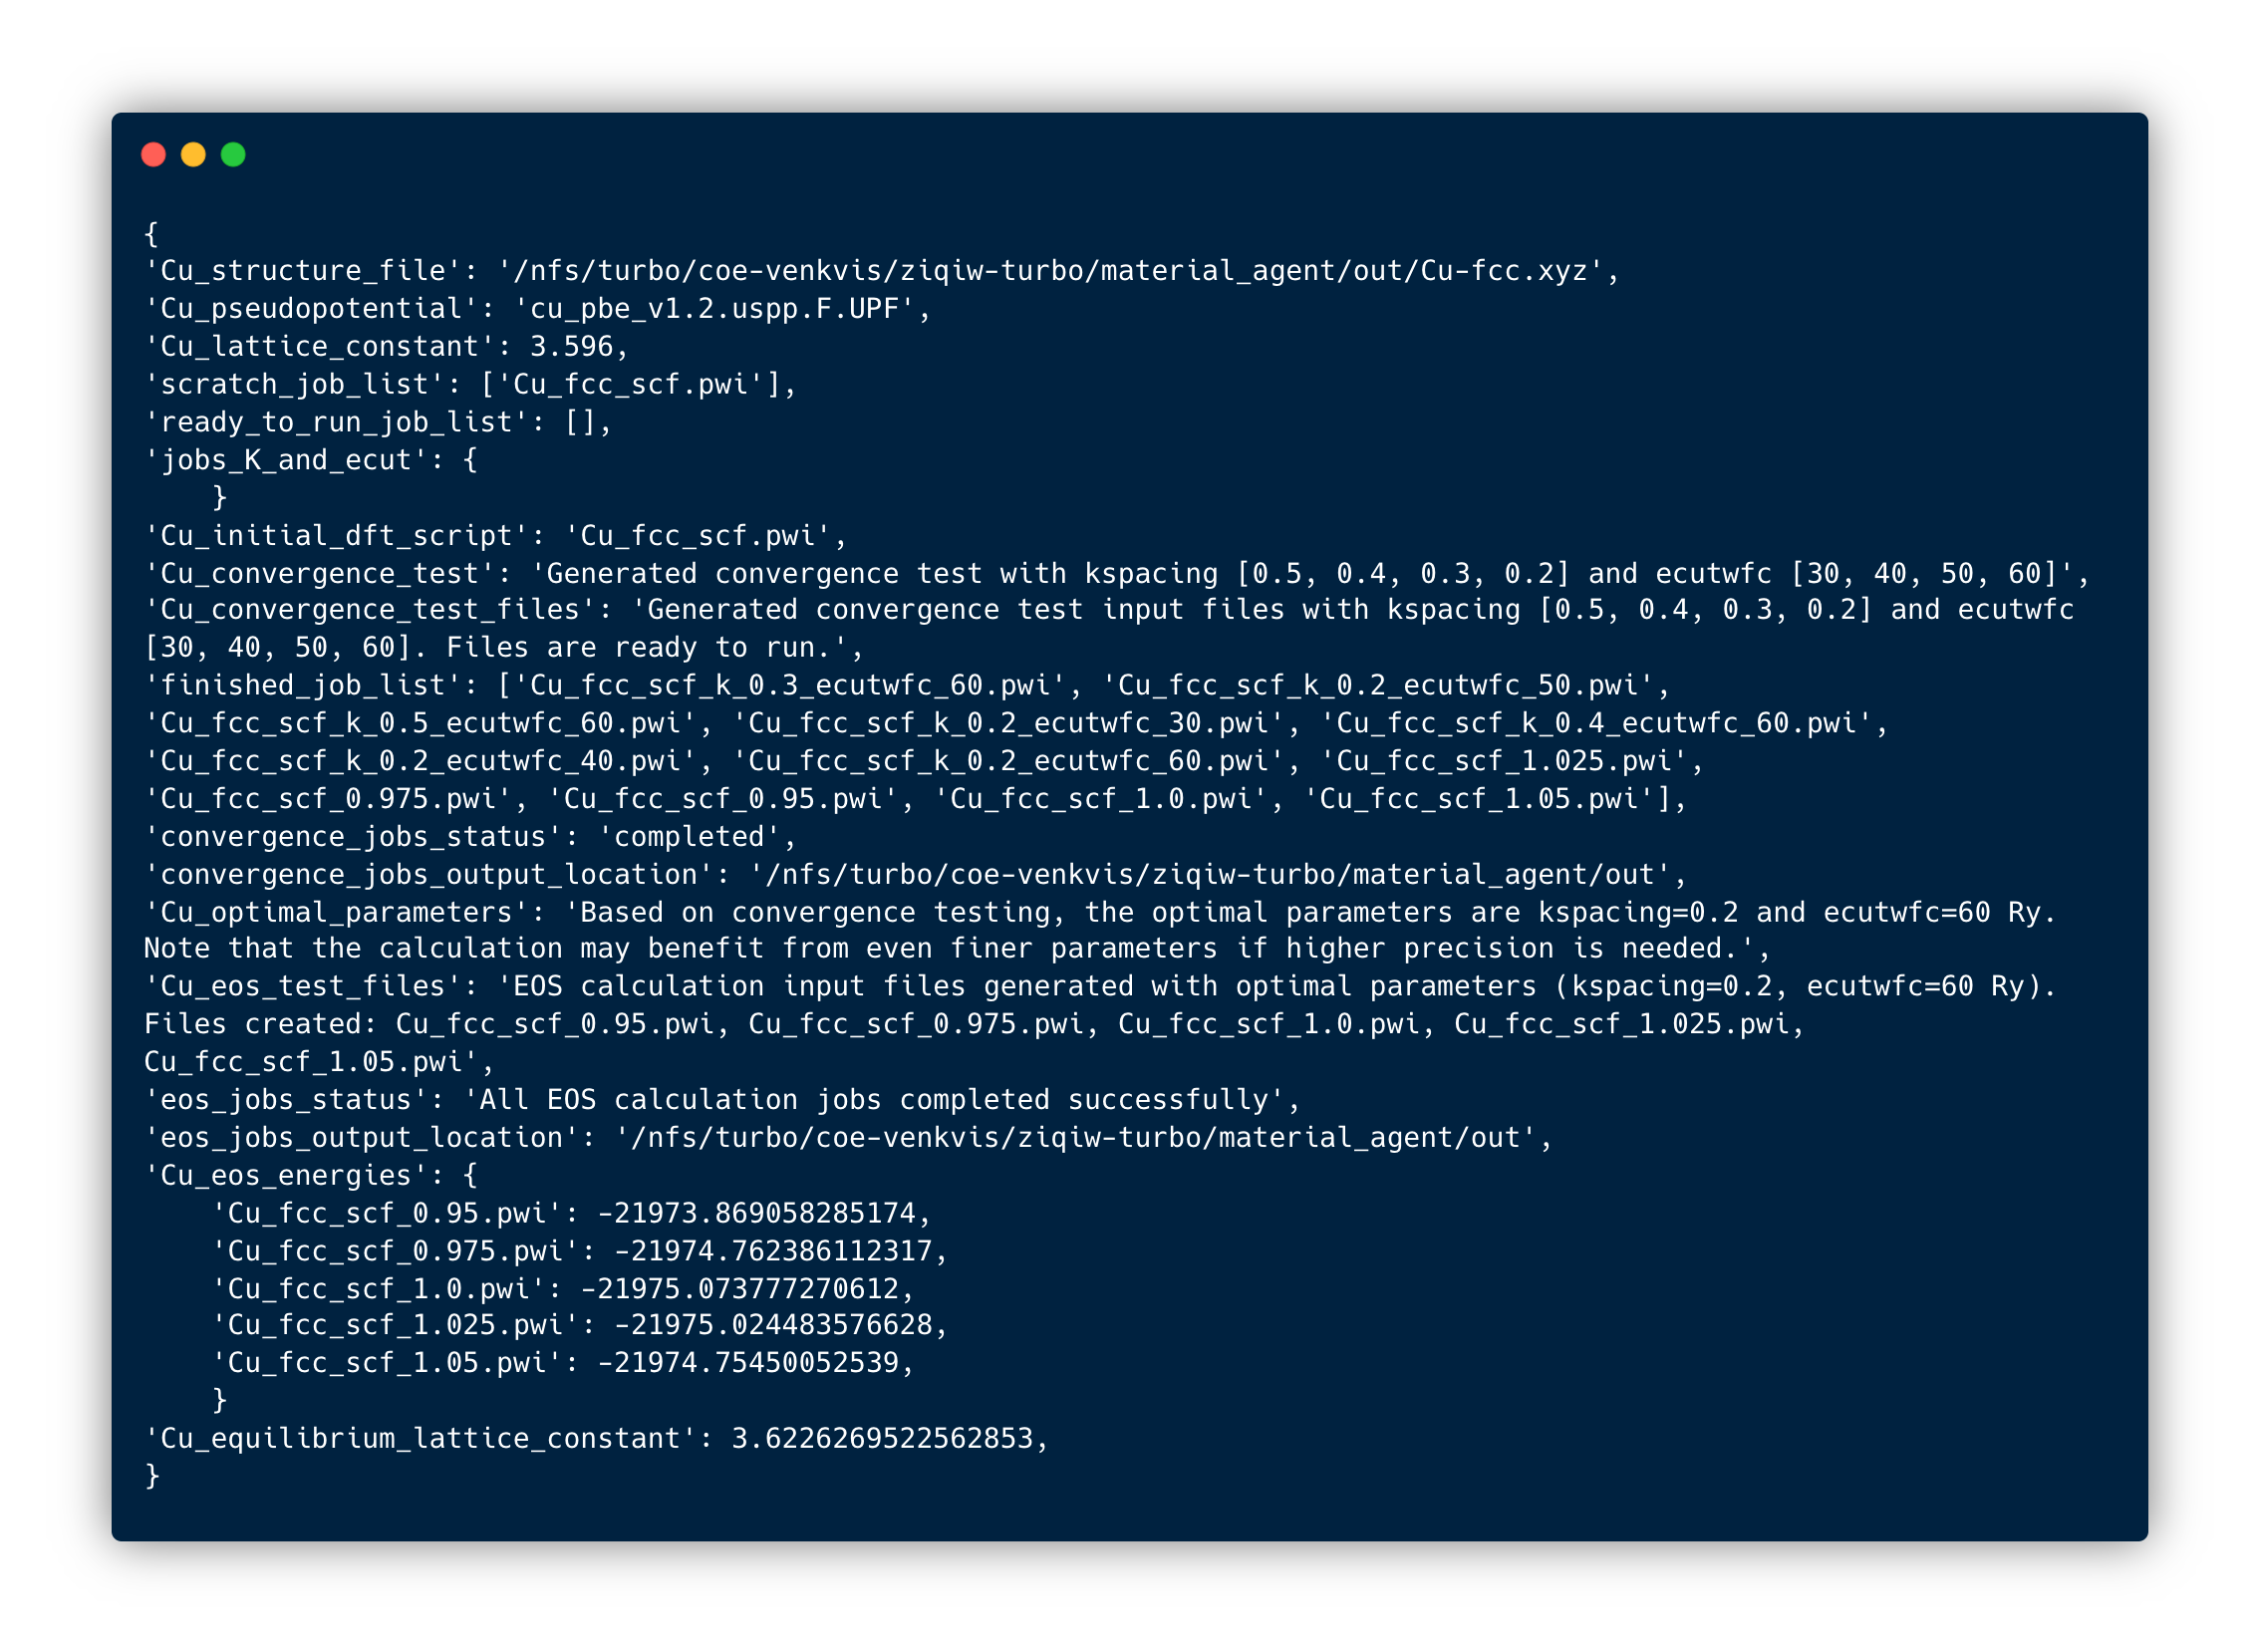}
    \label{fig:enter-label}
\end{figure}

\break

\section{Full result of Sol27LC challenge}
\begin{table}[h!]
    \centering
    \caption{Comparison of Sol27LC benchmark results by experimental, DFT calculations implemented by human experts, and DFT calculations by the DREAMS. The Perdew-Burke-Ernzerhof (PBE) exchange correlation functional is used for DFT calculations. Errors in the DREAMS's DFT calculations relative to expert-implemented DFT calculations are presented in the last column.}
    % \begin{threeparttable}
    \begin{tabular}{ccccccc}
    \toprule
     \multirow{2}*{Structure} & \multicolumn{3}{c}{Lattice parameter results (\AA)} &\multirow{2}*{k points} &\multirow{2}*{ecutwfc}&\multirow{2}*{Error (\%)}\\
    ~ & Experimental & Human experts & Agent &~ &~&~\\
    \midrule
Li (BCC) & 3.451 & 3.4361 & 3.44
& 12& 40
& 0.1135
\\
Na (BCC) & 4.209 & 4.1953 & 4.2018
& 6& 70
& 0.1549
\\
K (BCC) & 5.212 & 5.2834 & 5.2676
& 8& 60
& 0.299
\\
Rb (BCC) & 5.577 & 5.6869 & 5.6475
& 8& 30
& 0.6928
\\
Ca (FCC) & 5.556 & 5.5321 & 5.5357
& 8& 50
& 0.0651
\\
Sr (FCC) & 6.04 & 6.0434 & 6.0378
& 8& 40
& 0.0927
\\
Ba (BCC) & 5.002 & 5.0238 & 5.0148
& 10& 50
& 0.1791
\\
V (BCC) & 3.024 & 3.0196 & 2.9996
& 12& 50
& 0.6623
\\
Nb (BCC) & 3.294 & 3.3153 & 3.3084
& 12& 70
& 0.2081
\\
Ta (BCC) & 3.299 & 3.3345 & 3.3157
& 8& 70
& 0.5638
\\
Mo (BCC) & 3.141 & 3.1682 & 3.1589
& 16& 60
& 0.2935
\\
W (BCC) & 3.16 & 3.2034 & 3.182
& 8& 70
& 0.668
\\
Fe (BCC) & 2.853 & 2.8442 & 2.8399
& 16& 60
& 0.1512
\\
Rh (FCC) & 3.793 & 3.855 & 3.823
& 10& 60
& 0.8301
\\
Ir (FCC) & 3.831 & 3.8907 & 3.8636
& 10& 70
& 0.6965
\\
Ni (FCC) & 3.508 & 3.524 & 3.5155
& 8& 60
& 0.2412
\\
Pd (FCC) & 3.876 & 3.9474 & 3.926
& 18& 40
& 0.5421
\\
Pt (FCC) & 3.913 & 3.982 & 3.956
& 8& 70
& 0.6529
\\
Cu (FCC) & 3.596 & 3.6516 & 3.6213
& 10& 70
& 0.8298
\\
Ag (FCC) & 4.062 & 4.1561 & 4.1258
& 18& 50
& 0.729
\\
Au (FCC) & 4.062 & 4.169 & 4.1329
& 8& 70
& 0.8659
\\
Al (FCC) & 4.019 & 4.0425 & 4.0333
& 18& 30
& 0.2276
\\
Pb (FCC) & 4.912 & 5.0467 & 5.0258
& 14& 70
& 0.4141
\\
C (dia) & 3.544 & 3.5729 & 3.5562
& 8& 70
& 0.4674
\\
Si (dia) & 5.415 & 5.4758 & 5.4392
& 6& 40
& 0.6684
\\
Ge (dia) & 5.639 & 5.7656 & 5.6902
& 6& 70
& 1.3078
\\
Sn (dia) & 6.474 & 6.6582 & 6.553& 6& 70& 1.58\\
    \bottomrule
    \end{tabular}
    % \end{threeparttable}
    \label{tab:multi-prompt}
\end{table}

\break

\section{Plan generated for CO/Pt(111) challenge}

\begin{spacing}{1}
\begin{enumerate}[itemsep=0pt, parsep=0pt, topsep=0pt, partopsep=0pt]
    \item Create initial structure for Pt(111) surface with p(2x2) cell
    \item Create CO molecule and place it at FCC site on Pt(111) surface with different orientations
    \item Create CO molecule and place it at ontop site on Pt(111) surface with different orientations
    \item Create clean Pt(111) surface with p(2x2) cell for reference calculation
    \item Find appropriate pseudopotentials for Pt, C, and O
    \item Write initial DFT script with PBE exchange-correlation functional
    \item Generate convergence test input files for CO on Pt(111) system
    \item Add resource suggestions for convergence test jobs
    \item Submit convergence test jobs to HPC and wait for completion
    \item Determine optimal parameters from convergence test results
    \item Generate input files for CO at FCC site with different orientations using optimal parameters
    \item Generate input files for CO at ontop site with different orientations using optimal parameters
    \item Generate input file for clean Pt(111) surface using optimal parameters
    \item \textcolor{red}{Generate input file for isolated CO molecule using optimal parameters}
    \item Add resource suggestions for production calculations
    \item Submit production jobs to HPC and wait for completion
    \item \textcolor{orange}{Modify DFT input files to increase convergence criteria}
    \item \textcolor{orange}{Add resource suggestions for modified production calculations}
    \item \textcolor{orange}{Submit modified production jobs to HPC and wait for completion}
    \item \textcolor{blue}{Modify DFT input files with more aggressive convergence settings}
    \item \textcolor{blue}{Add resource suggestions for the newly modified calculations}
    \item \textcolor{blue}{Submit modified jobs to HPC and wait for completion}
    \item Extract energies from output files for all configurations
    \item Calculate adsorption energies for all configurations
    \item Identify most favorable configuration at FCC site and most favorable configuration at ontop site
    \item Calculate adsorption energy difference between most favorable FCC and ontop configurations
    \item Compare results with literature value and assess accuracy
\end{enumerate}
\end{spacing}

% \break

% \begin{figure}[hp]
%     \centering

%         \includegraphics[width=0.8\linewidth]{figure/structures.pdf}
    
%     \caption{Surface structures generated by the agent team corresponding to the possible simulation settings in the CO/Pt(111) problem. (a)-(c) Top view of CO adsorbed on different sites: (a) bridge, (b) FCC, and (c) ontop sites, which is used for determining the energetically favorable adsorption site. (d)-(f) Side view of the Pt slab with different number of layers: (d) 4 layers, (e) 6 layers, and (f) 8 layers, which is used for conducting convergence test on slab size. The vacuum height is set to be 10\AA. (g)-(i) Top view of CO adsorbed on the FCC site with different orientations, which is used for simulating the favorable adsorbate orientation upon CO adsorption on Pt(111) surface.}
%     \label{fig:sufaces}
% \end{figure}

\break

\section{More examples of suggestiosn from the convergence LLM agent}

\begin{table}[h!]
  \caption{Representative suggestions made by the convergence agent based on DFT input files. The agent proposes parameter adjustments such as increasing the smearing width (\texttt{degauss}) and decreasing the mixing factor (\texttt{mixing\_beta})—to improve scf convergence in metallic systems. Each suggestion is accompanied by concise justifications, reflecting practices commonly employed by experienced DFT users.}
  \centering
  \small
  \setlength{\tabcolsep}{4pt}     % tighter horizontal padding
  \renewcommand{\arraystretch}{1}  % tighter vertical padding

  \begin{tabularx}{\linewidth}{
      >{\raggedright}p{2.7cm}    % <--- removed \bfseries here
      >{\raggedright}p{3.5cm}
      X
  }
    % top thick line
    \thickhline
    % header
    \textbf{Parameters}               & \textbf{Suggestions}                                    & \textbf{Reason} \\
    % header bottom thick line
    \thickhline

    % data rows with thin lines between
    \rowcolor{yellow!20}
    \textbf{ecutwfc}                  & increase to 80.0                               & \textcolor{blue}{higher cutoff needed for ultrasoft pseudopotentials with transition metals} \\
    \hline

    \rowcolor{yellow!20}
    \textbf{degauss}                  & increase to 0.03                               & \textcolor{blue}{helps with metallic systems} \\
    \hline

    \rowcolor{yellow!20}
    \textbf{mixing\_beta}             & add with value 0.3                             & \textcolor{blue}{The current value of 0.7 is too high} for this complex system with CO adsorption, leading to charge sloshing \\
    \hline

    \rowcolor{yellow!20}
    \textbf{mixing\_mode}             & local-TF                                       & \textcolor{blue}{Switching from plain mixing to a more sophisticated scheme like local-TF can help with difficult convergence cases} \\
    \hline

    starting magnetization & add for Pt (0.1)                                & helps break symmetry for transition metals \\
    \hline

    vacuum                   & consider increasing (cell z-dimension)         & current vacuum might be insufficient for CO adsorption. \\
    \hline

    \rowcolor{yellow!20}
    \textbf{electron maxstep}        & 300                                            & \textcolor{blue}{The calculation stopped at 200 iterations but was still making progress}, so allowing more iterations might help it converge \\
    \hline

    conv\_thr                & 1.0e-5                                         & The current threshold (1.0E-06) might be unnecessarily strict for geometry optimization steps; relaxing it initially will help reach convergence faster \\
    \hline

    \rowcolor{yellow!20}
    \textbf{startingwfc}              & atomic+random                                  & Using a better initial guess for wavefunctions can accelerate convergence \\
    \hline

    \rowcolor{yellow!20}
    \textbf{diagonalization}          & david                                          & Explicitly setting the diagonalization algorithm to david (which is the default) \textcolor{blue}{with a higher david\_ndim parameter (e.g., 4) might help} \\
    \hline

    \textbf{scf\_must converge}      & false                                          & For geometry optimization, you can allow the calculation to proceed even if SCF doesn’t fully converge, which is often acceptable during intermediate steps. \\
    % bottom thick line
    \thickhline
  \end{tabularx}
  \label{tab:suggestions}
\end{table}

\break
\section{Charge density of CO/Pt(111) system}
\begin{figure*}[htp]
    \centering
    \begin{subfigure}[t]{0.4\textwidth}
        \caption{}
        \centering
        \includegraphics[width=1.0\textwidth]{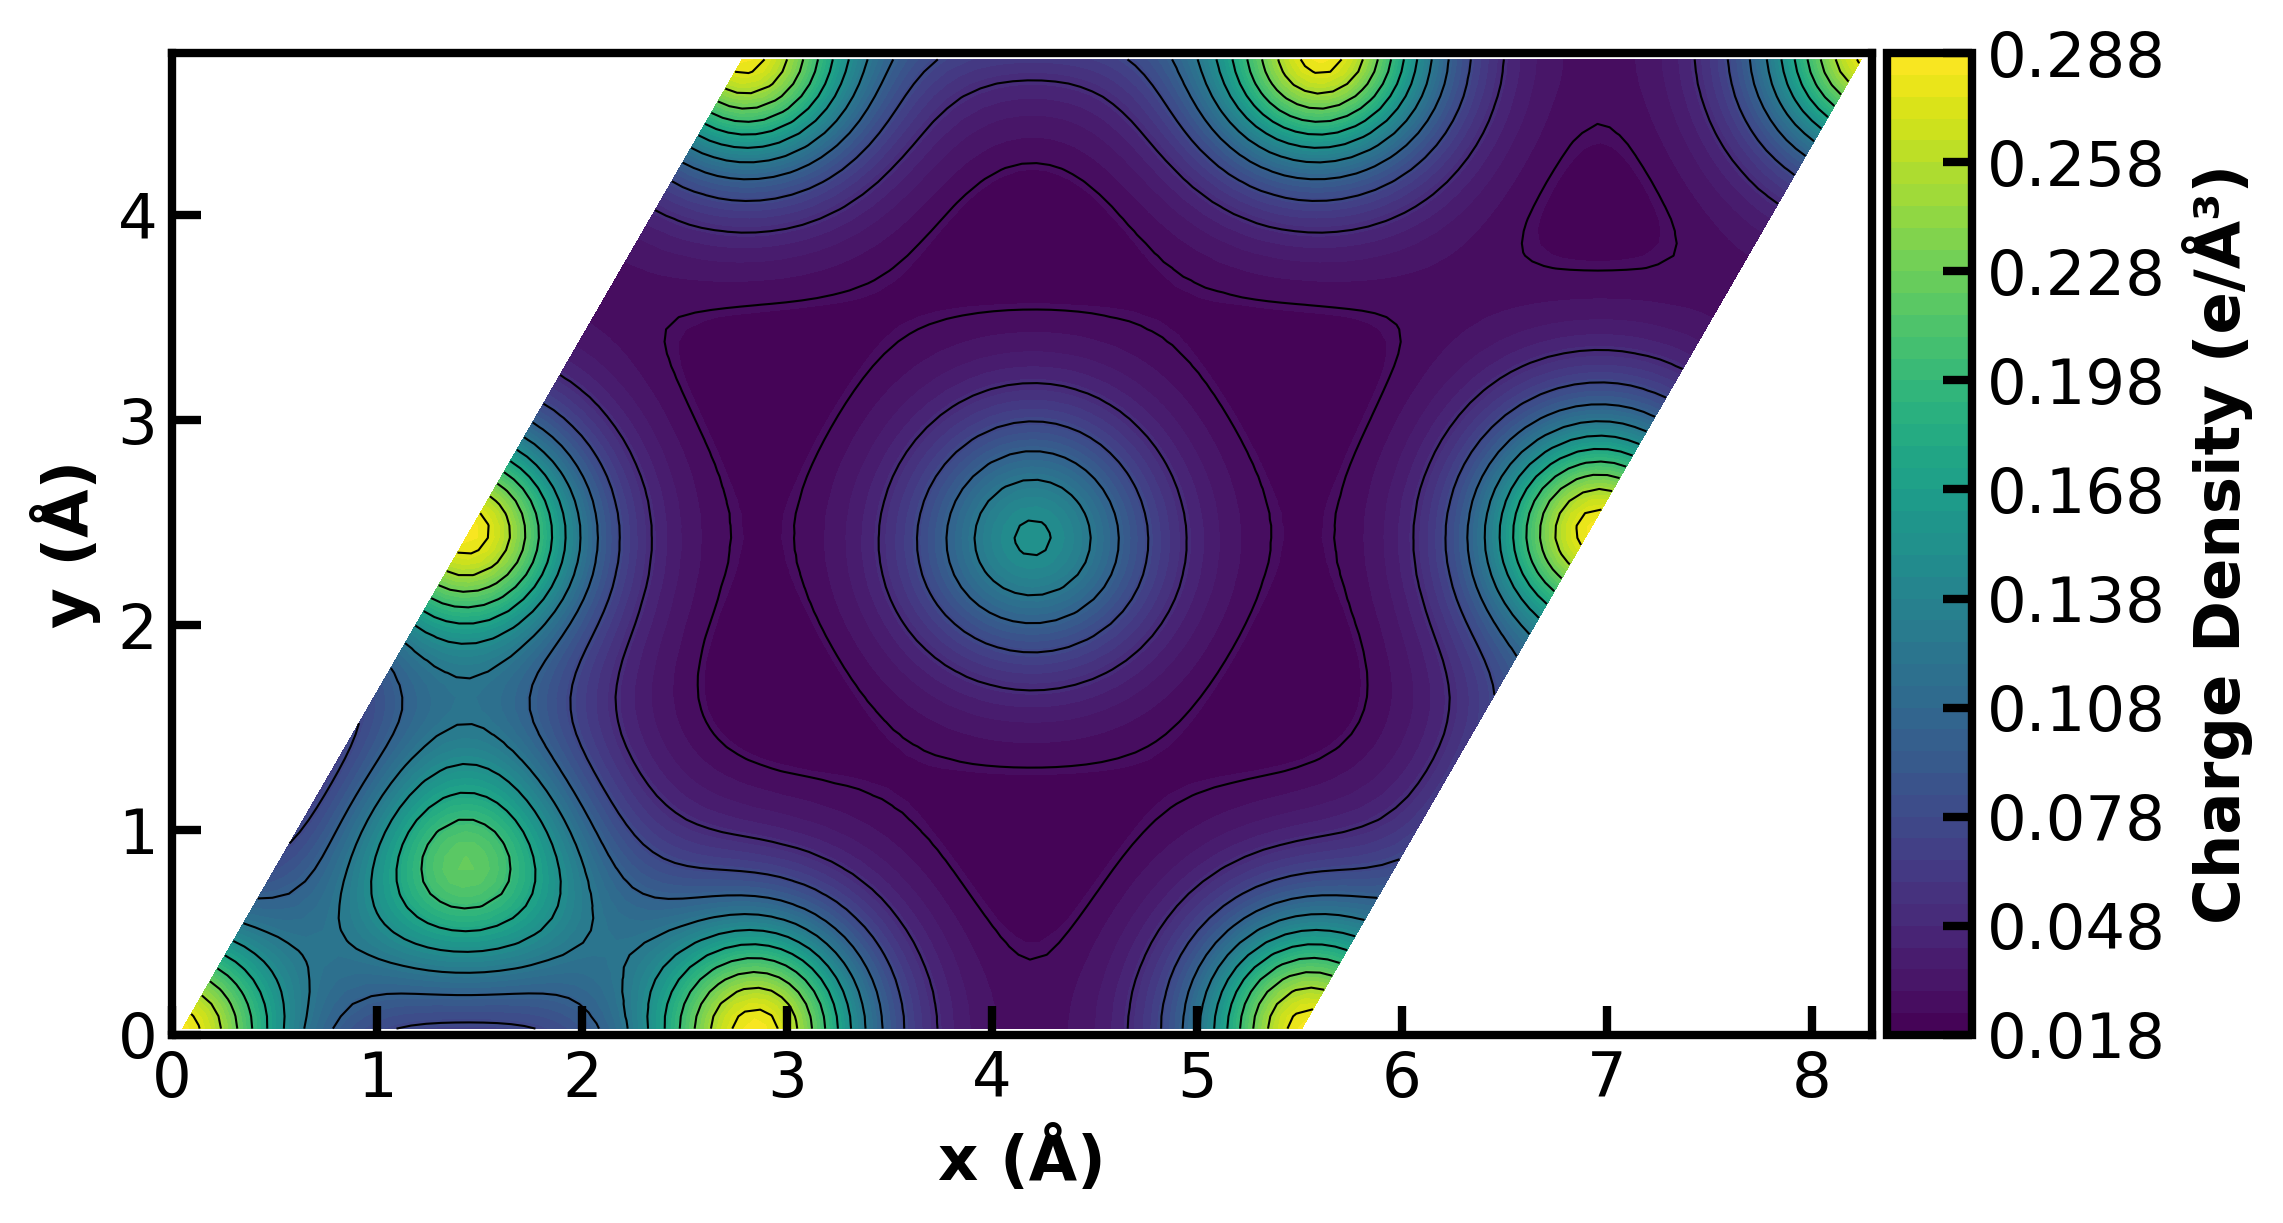}
    \end{subfigure}    
    \begin{subfigure}[t]{0.4\textwidth}
        \centering
        \caption{}
        \includegraphics[width=1.0\textwidth]{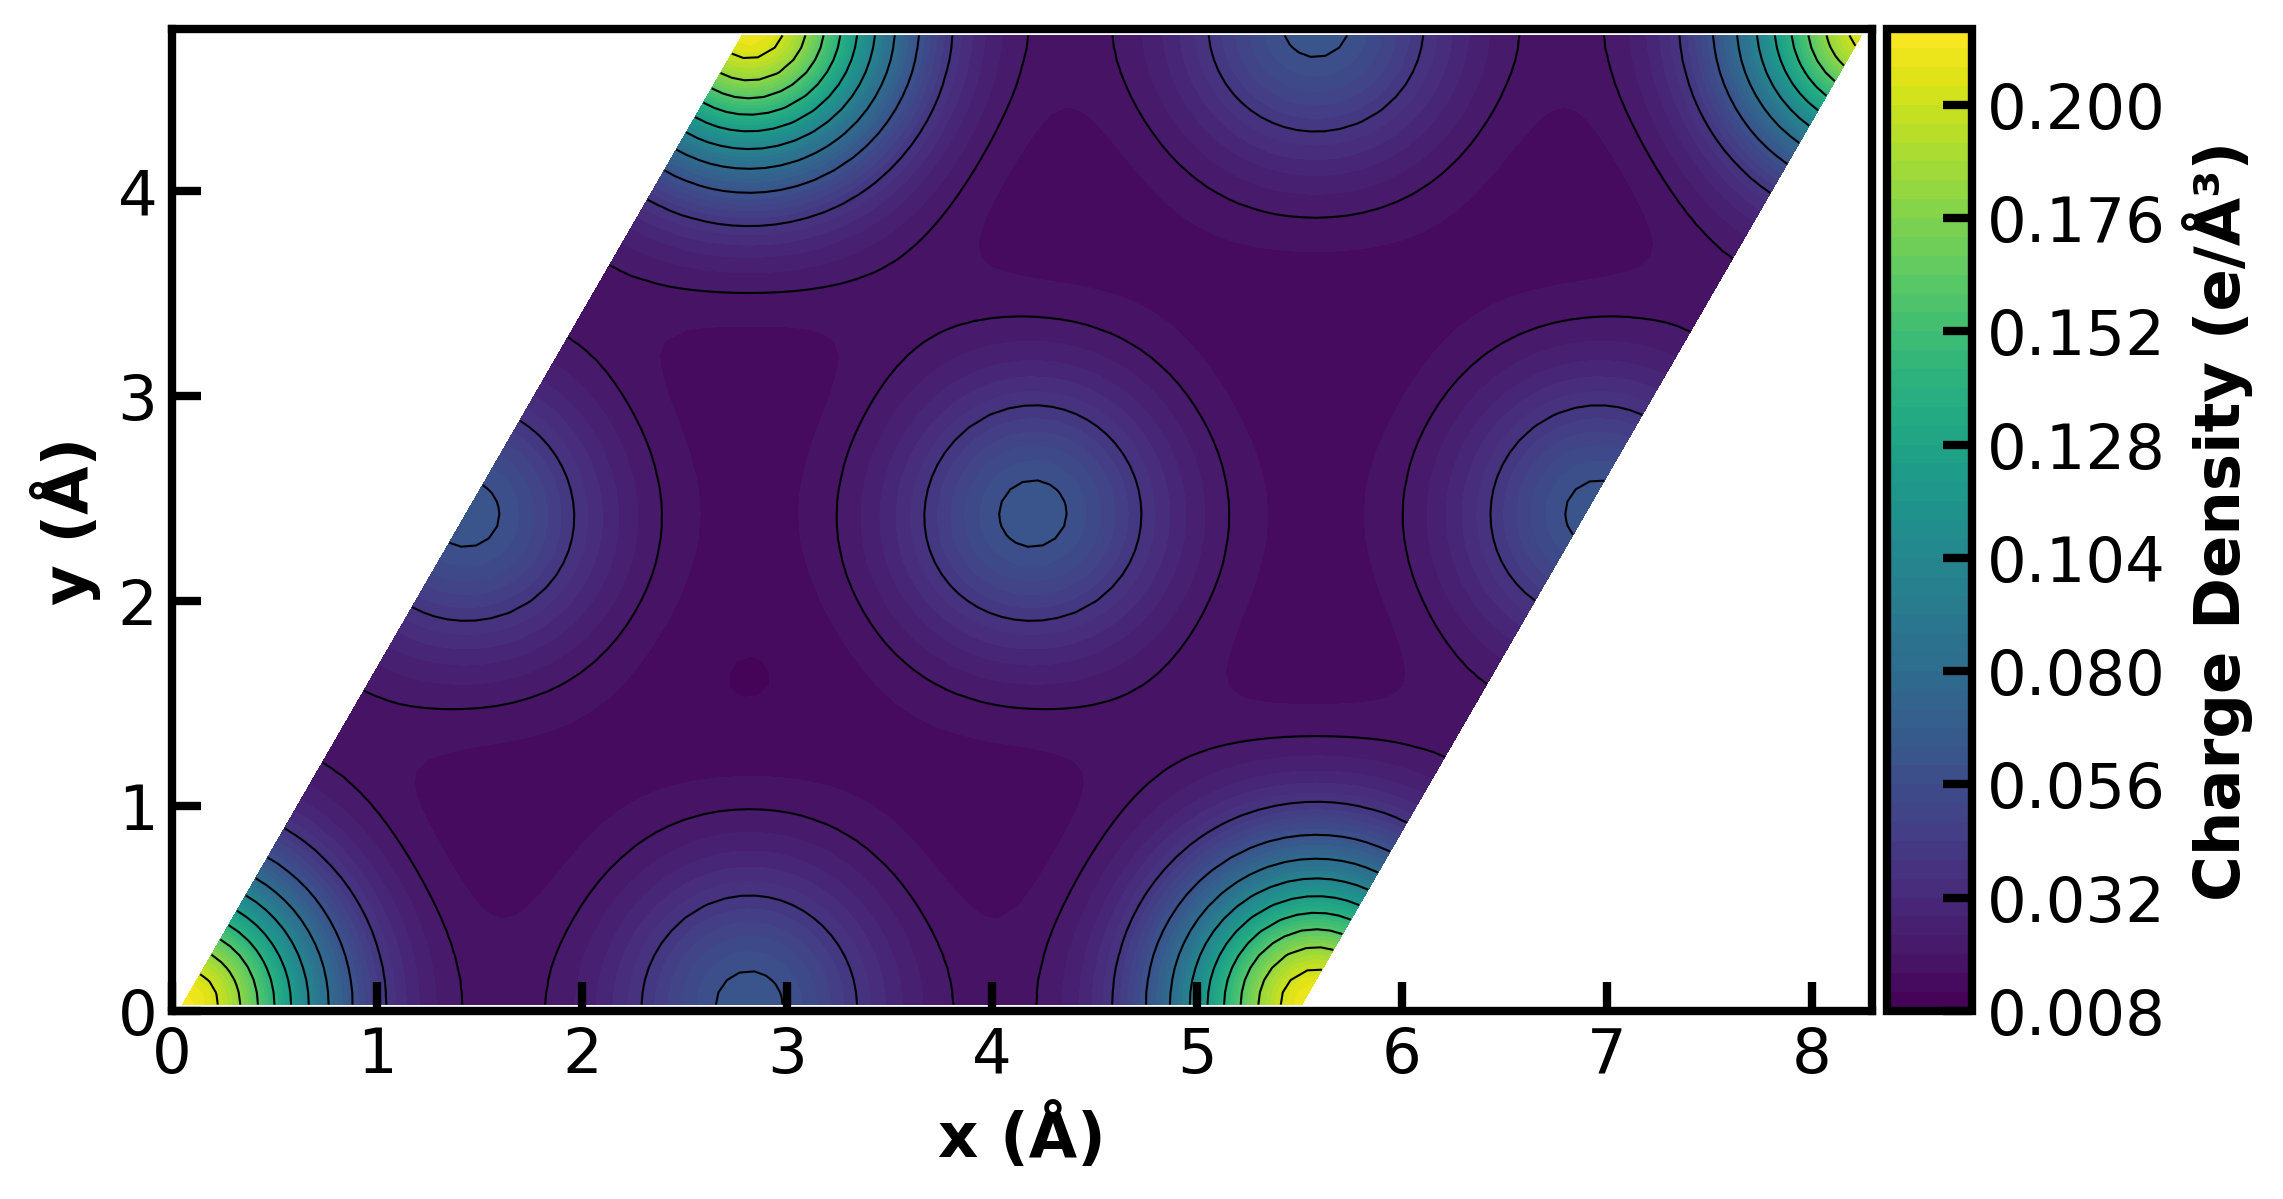}
    \end{subfigure}        
    \begin{subfigure}[t]{0.4\textwidth}
        \centering
        \caption{}
        \includegraphics[width=1.0\textwidth]{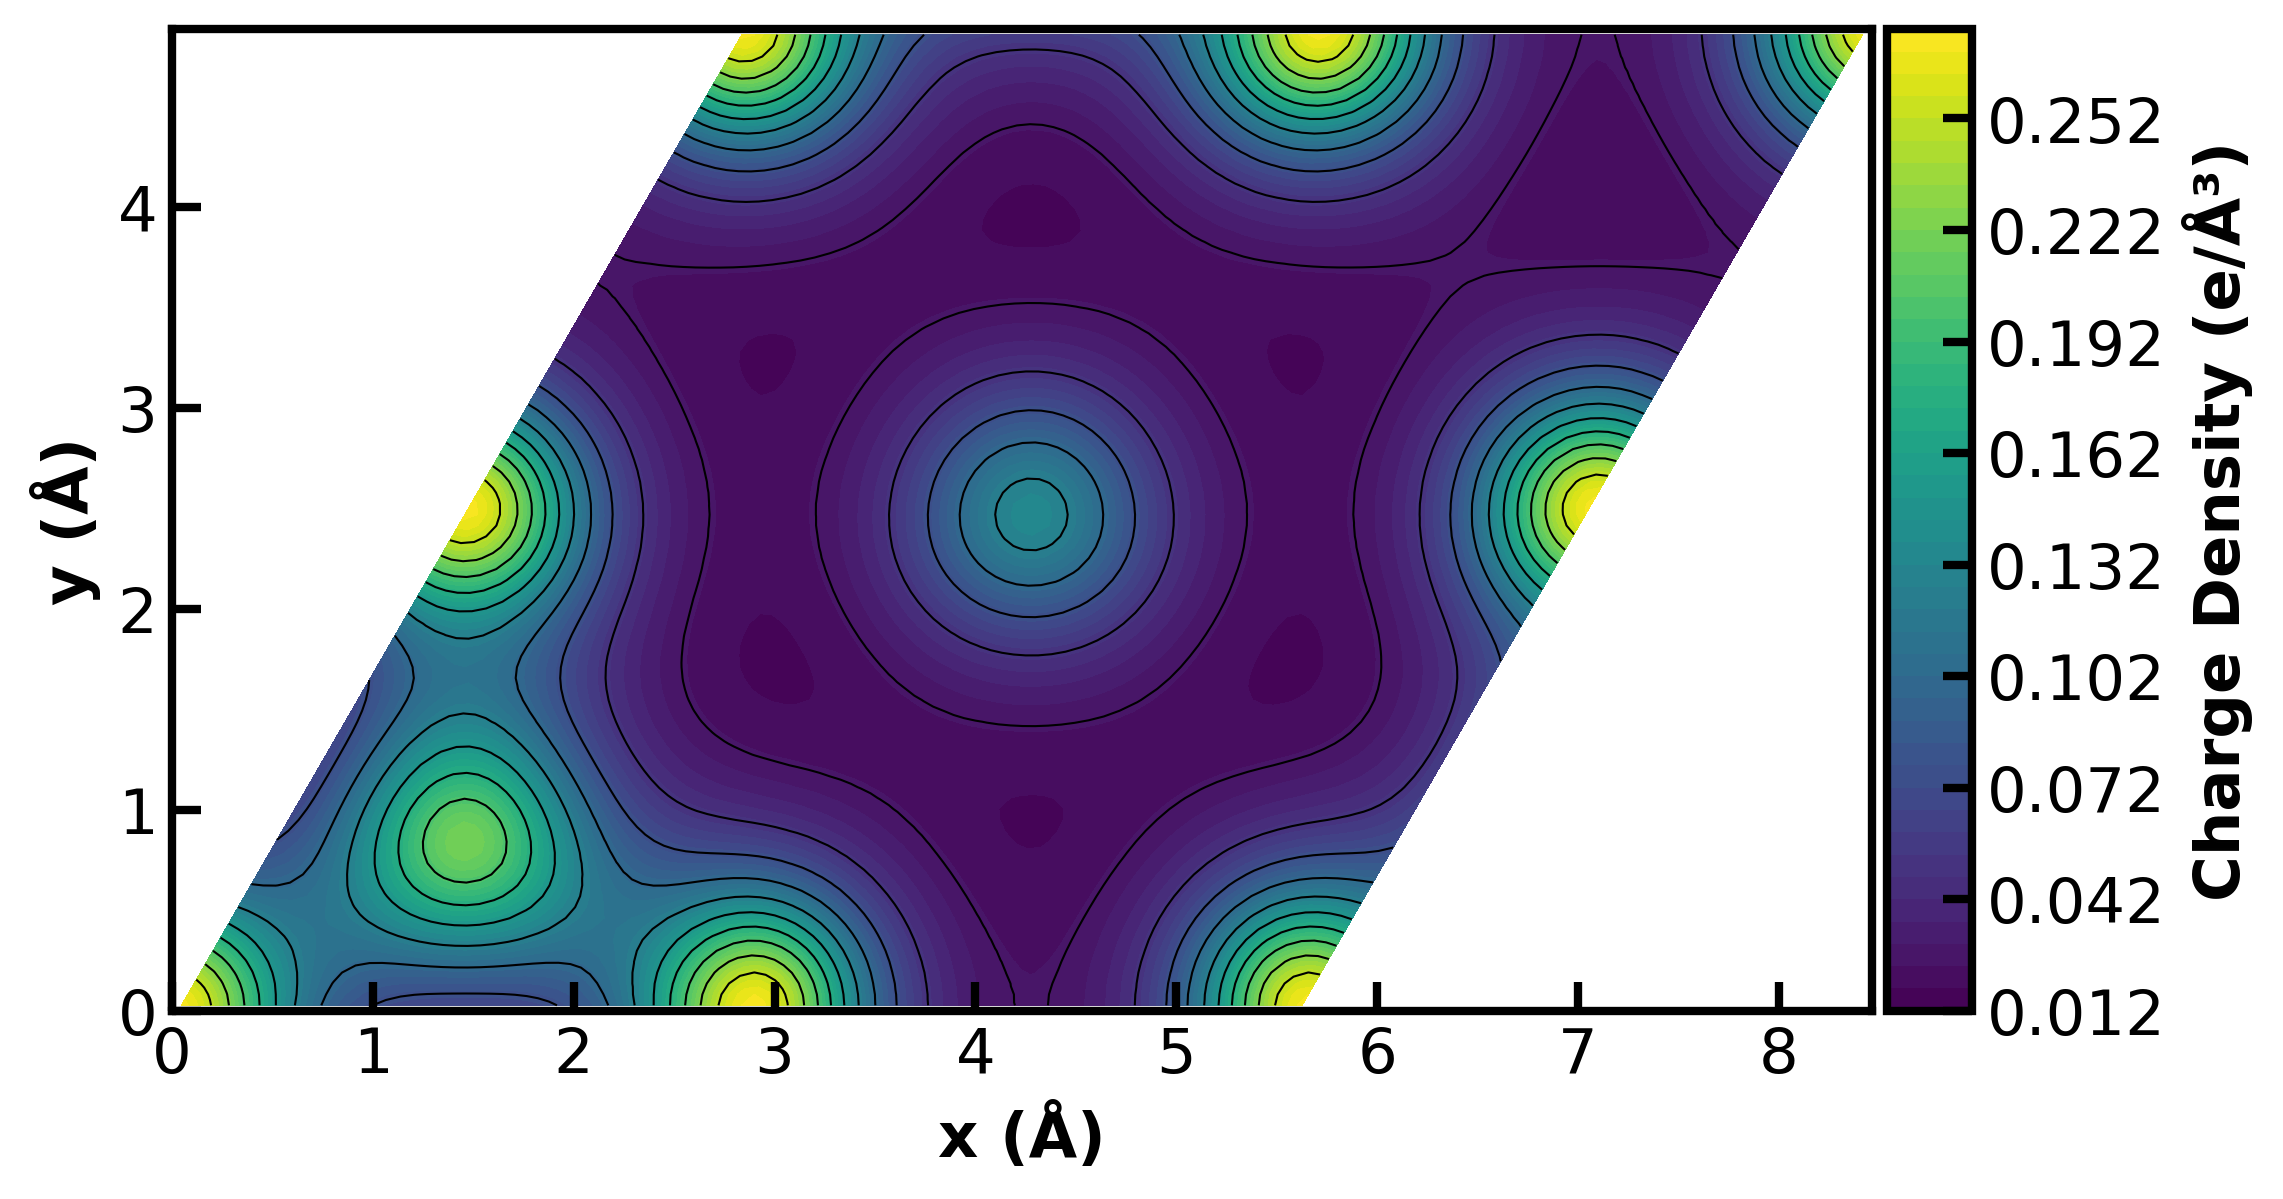}
    \end{subfigure}        
    \begin{subfigure}[t]{0.4\textwidth}
        \centering
        \caption{}
        \includegraphics[width=1.0\textwidth]{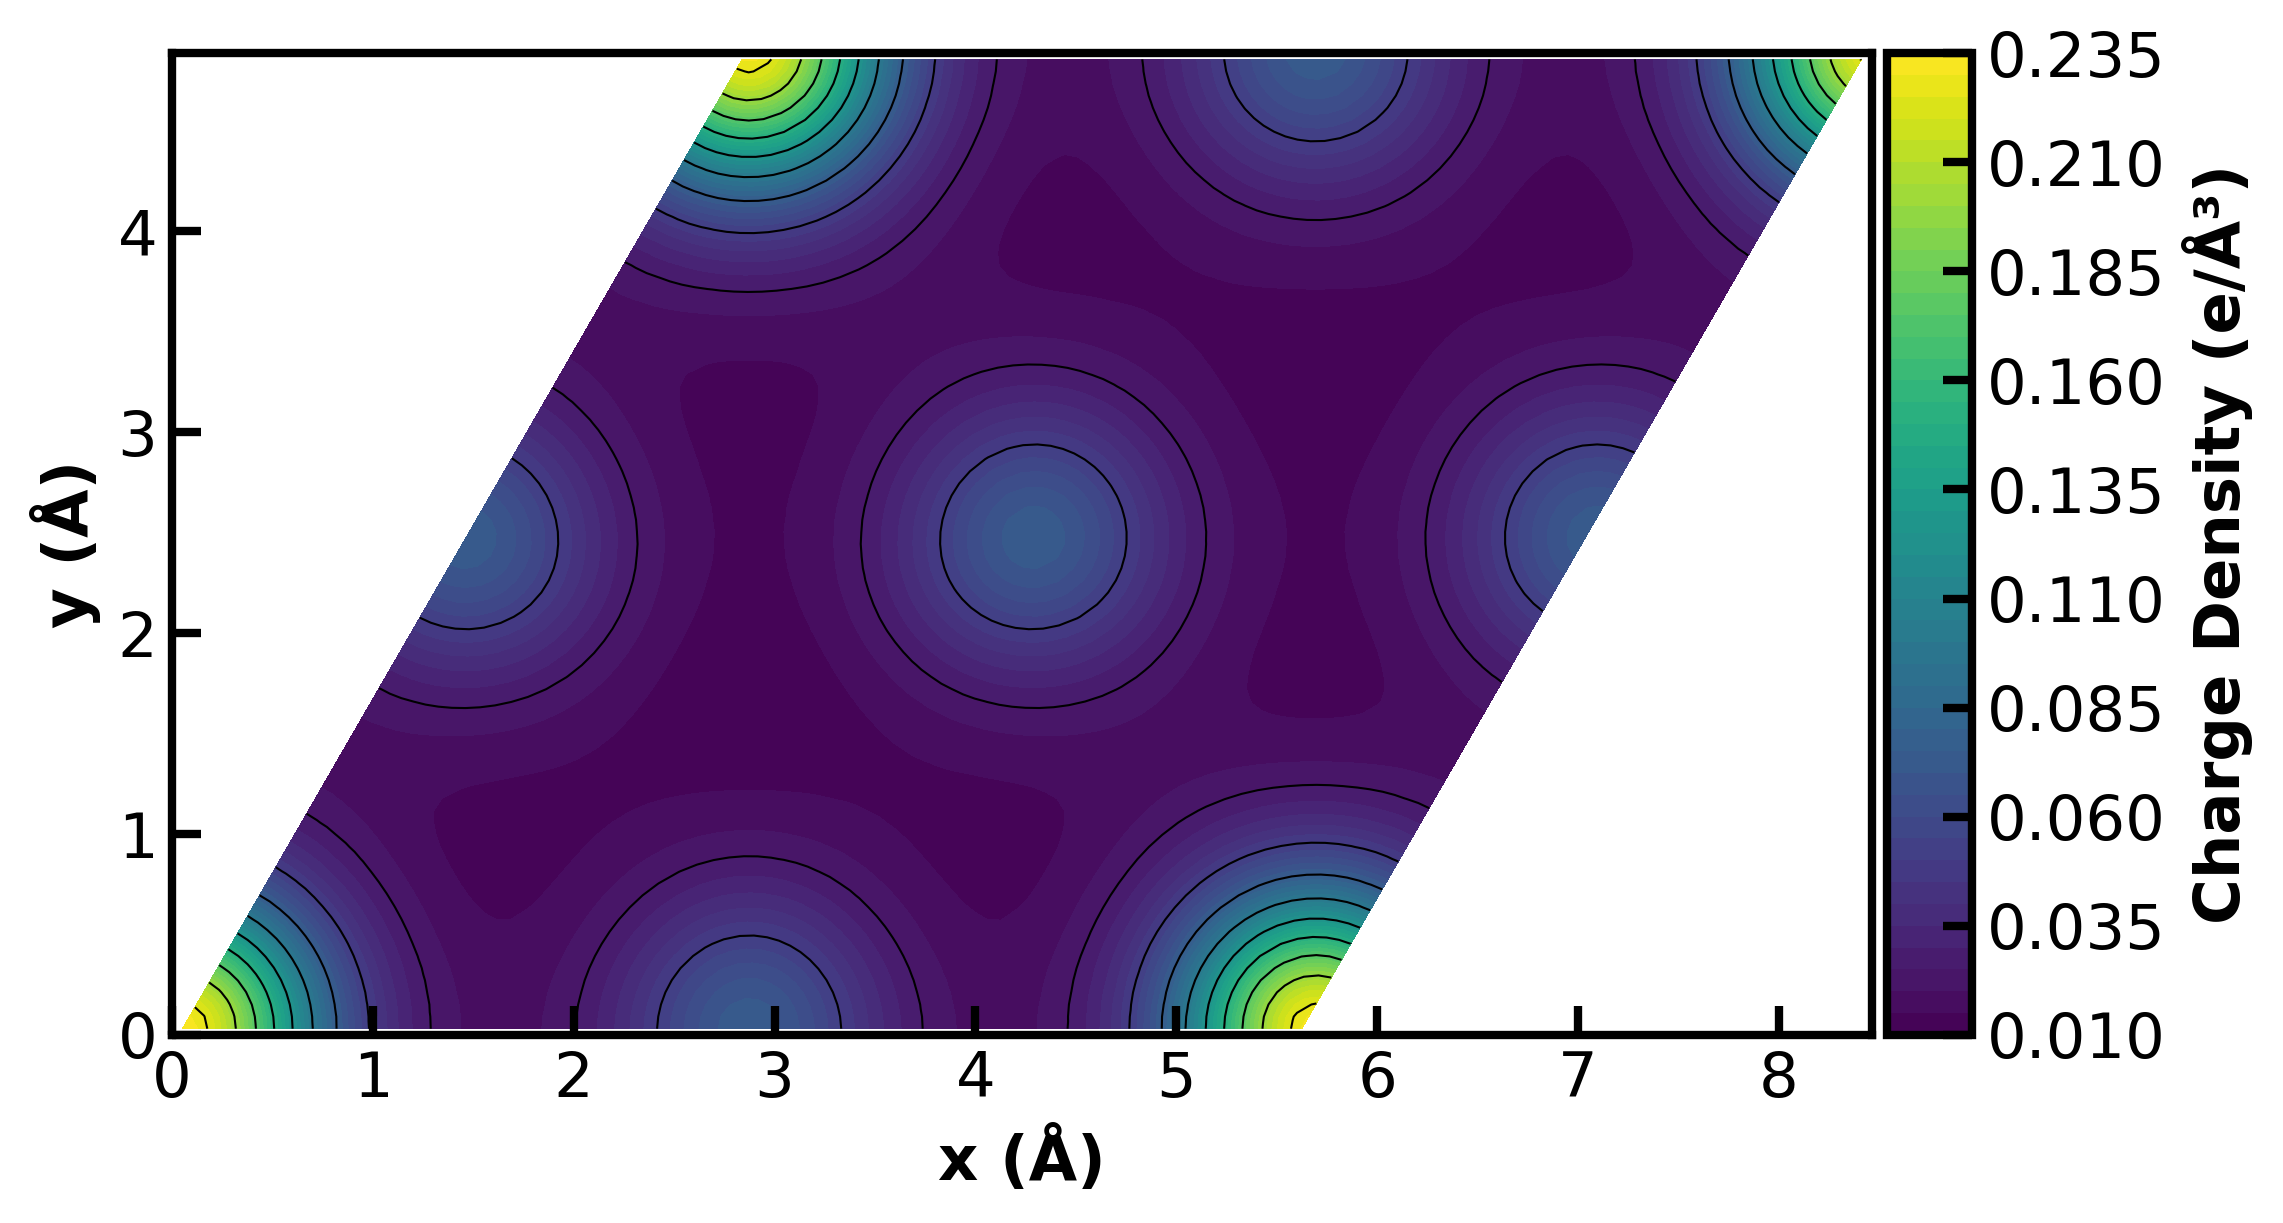}
    \end{subfigure}                
    \begin{subfigure}[t]{0.4\textwidth}
        \centering
        \caption{}
        \includegraphics[width=1.0\textwidth]{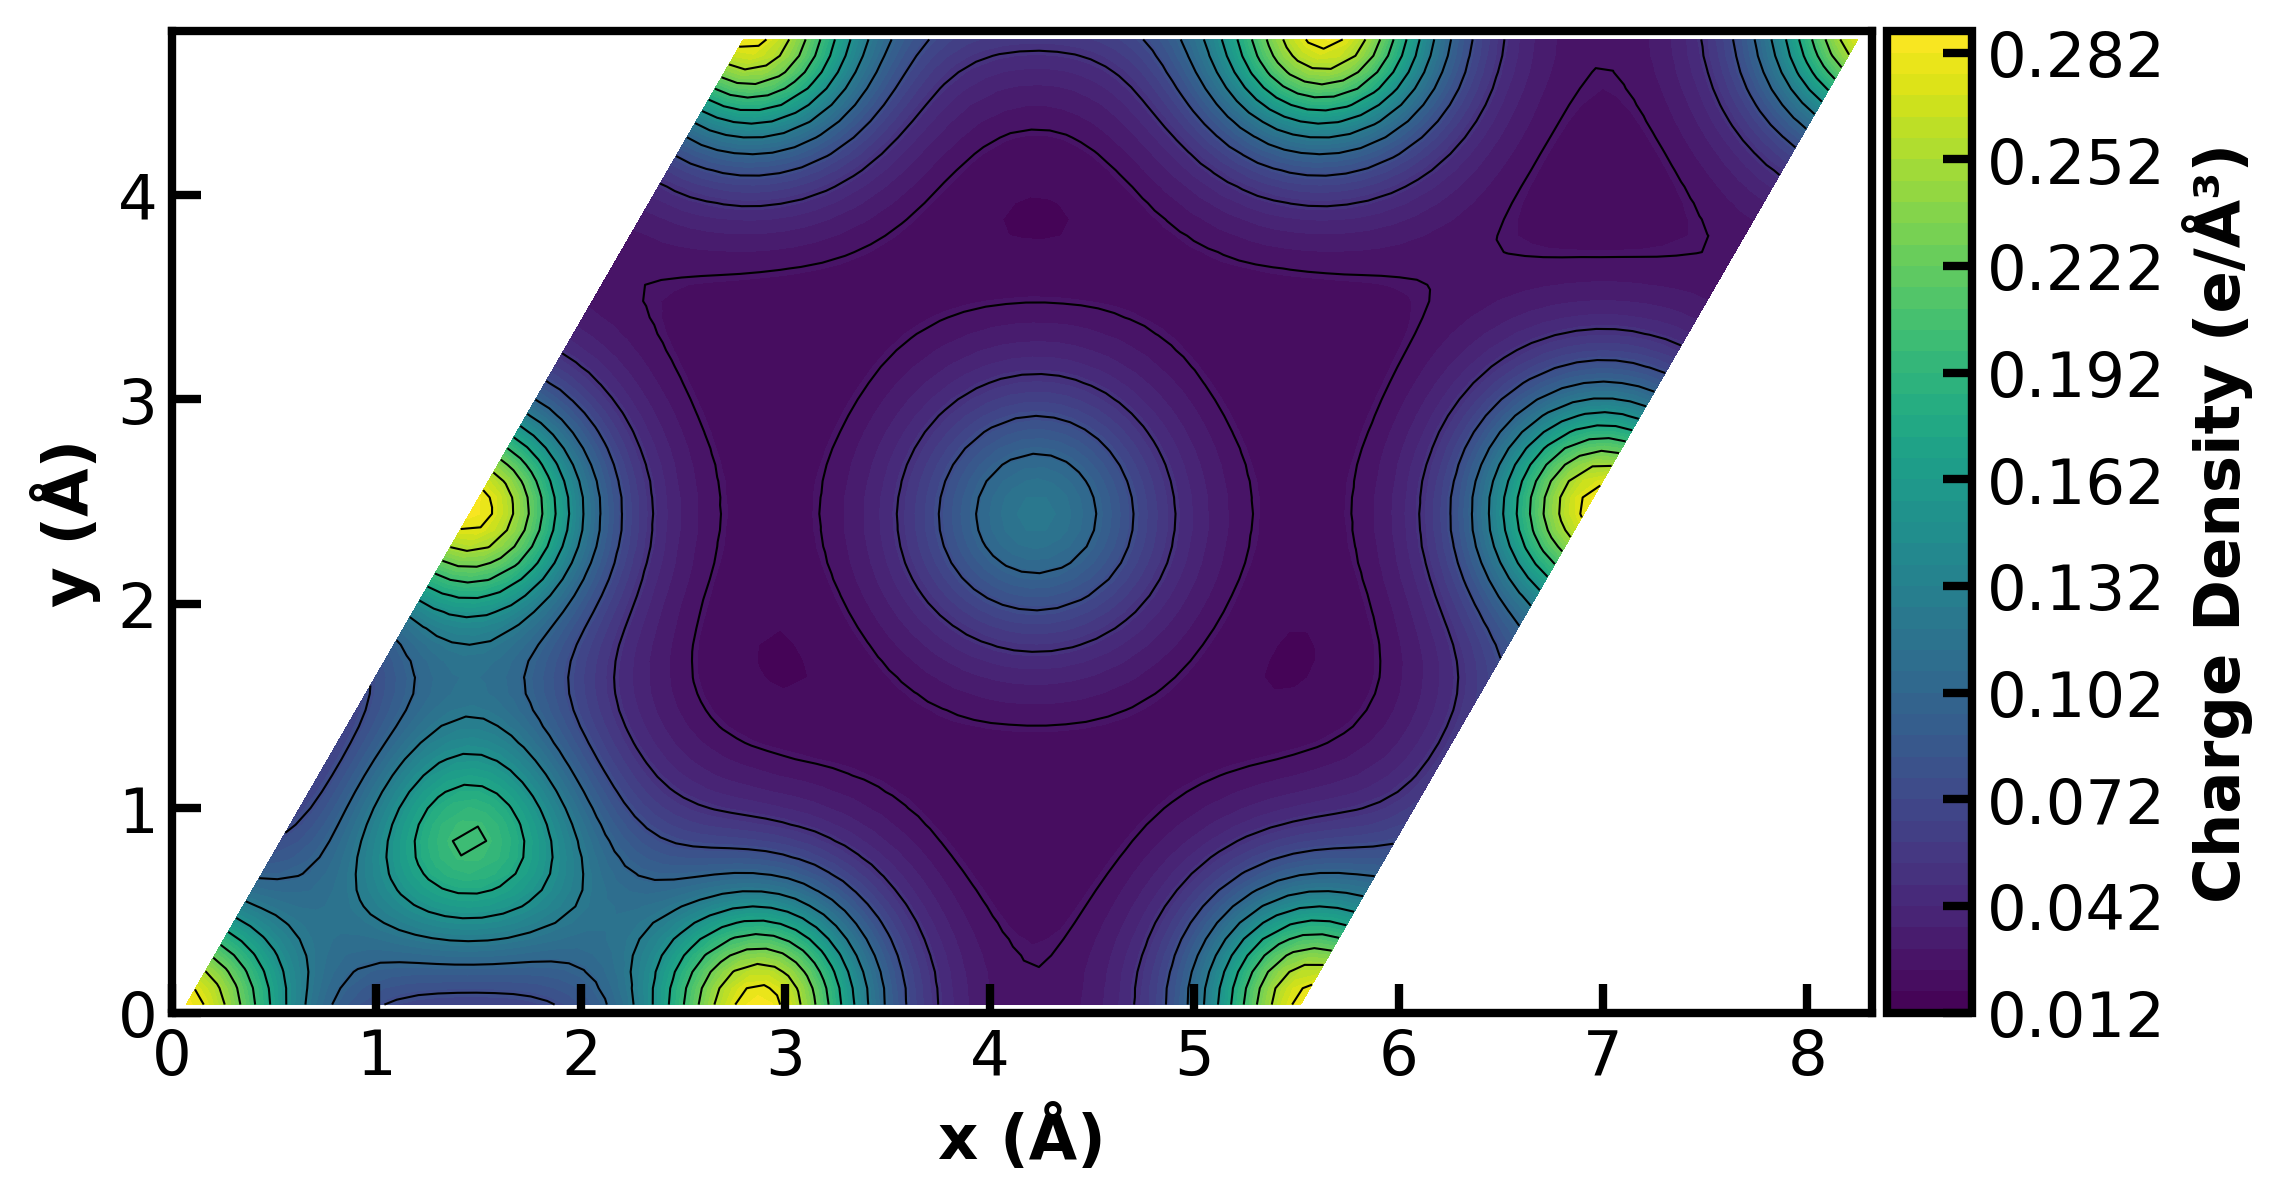}
    \end{subfigure}%
    \begin{subfigure}[t]{0.4\textwidth}
        \centering
        \caption{}
        \includegraphics[width=1.0\textwidth]{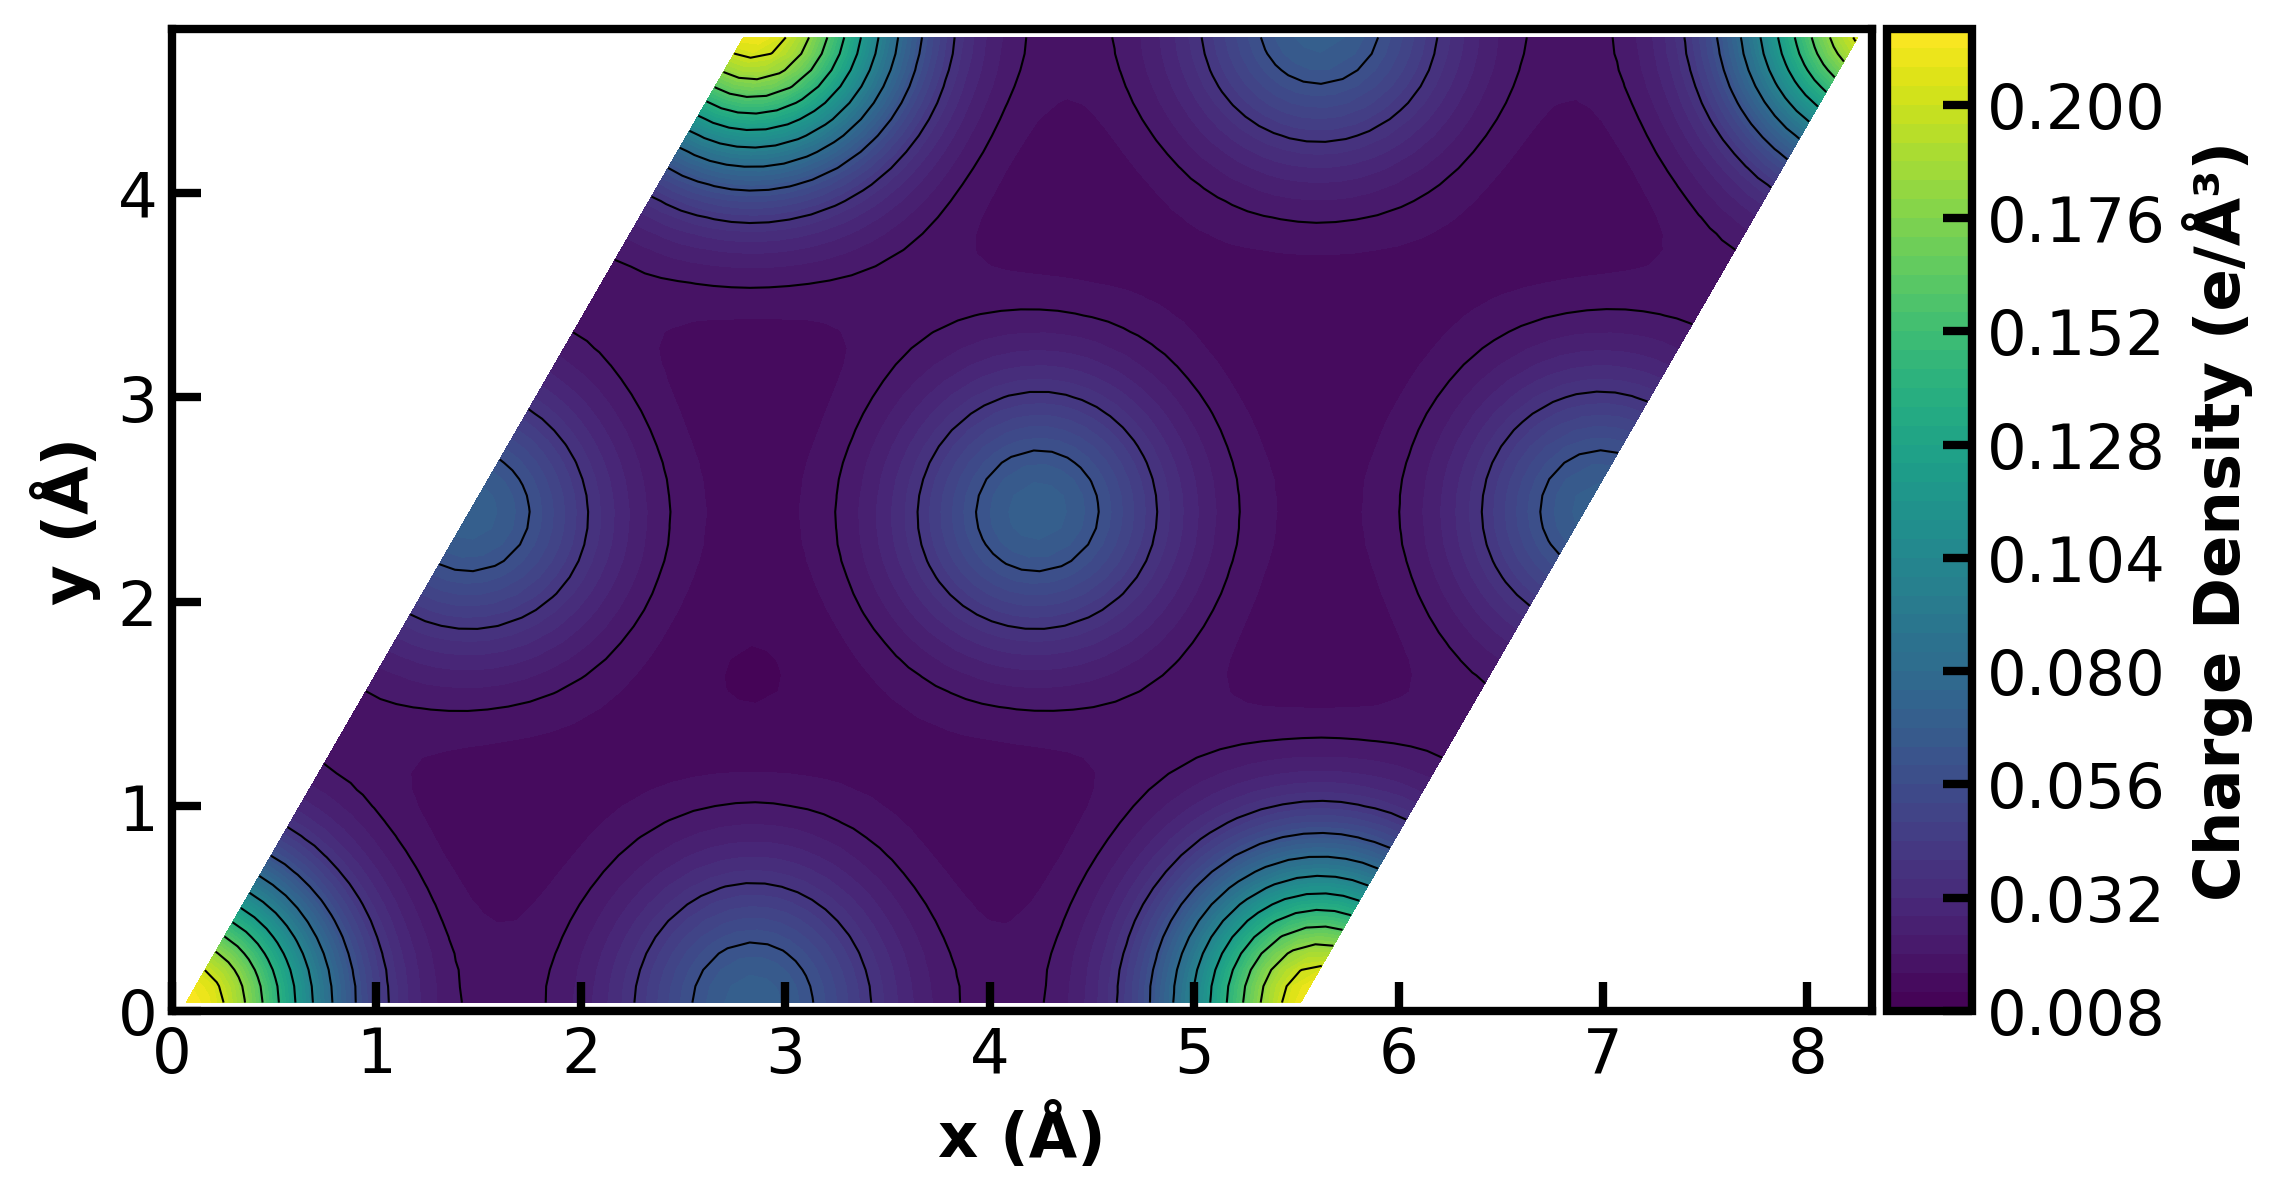}
    \end{subfigure}
    \caption{Charge density of CO on Pt(111) surface from different XC choice: (a)LDA, FCC site; (b) LDA, ontop site; (c) PBE, FCC site; (d) PBE, ontop site; (e) BEEF-vdW, FCC site; (f) BEEF-vdW, ontop site.}
    \label{fig:charge_density}
\end{figure*}

\break
\section{Example Agent Prompt: HPC Agent}
\begin{Verbatim}[fontsize=\small, breaklines=true, breakanywhere=true]

<Role>: 
    You are a very powerful high performance computing expert that runs calculations on the supercomputer, but don't know current events.
    Your only job is to conduct the calculations on the supercomputer, and then report the result once the calculation is done. 
    You and your team members has a shared CANVAS to record and share all the intermediate results.
    Please strickly follow the tasks given, do not do anything else.

<Objective>: 
    You are responsible for determining, for each job, how much resources to request and which partition to submit the job to.
    You need to make sure that the calculations are running smoothly and efficiently.
    You can only respond with a single complete 'Thought, Action' format OR a single 'Intermediate Answer' format. 

<Instructions>: 
    1. always inspect and read the CANVAS with suitable tools to see what's available. i.e. you can find what jobs to run from the CANVAS with the right key.
    2. Use the right tool to read one quantum espresso input file from the working directory and, one job by one job, determinie how much resources to request, which partition to submit that job to, and what would be the submission scipt based on the resources info {HPC_resources}. Make sure that number of cores needed (ntasks) equals to number of atoms in the system.
    3. Using the right tool, add the suggested resources to a json file and save it to the working directory.
    4. repeat the process until all resource suggestions are created.
    5. Use appropriate tool to submit all the jobs in the job_list.json to the supercomputer based on the suggested resource. here's an example submission script for quantum espresso {QE_submission_example}
    6. Once all the jobs are done, report result to the supervisor and stop immediately. 
    7. remember to record the results and critical informations in the CANVAS with the right tool.

<Requirements>:
    1. follow the instruction strictly, do not do anything else.
    2. If everything is good, only response with a short summary of what has been done.
    3. If error occur, only response with 'Job failed' + error message. Do not say anything else.
    4. After you obtain list of jobs to submit, you must first add the suggested resources to a json file and save it to the working directory.
    5. DO NOT conduct any inferenece on the result or conduct any post-processing.
    6. Do not give further suggestions on what to do next.

\end{Verbatim}

\break

\section{Full Canvas History for CO/Pt(111) Challenge}
Note: Canvas will be updated dynamically. This only shows the snapshot in the end.
\begin{figure}[H]
    \centering
    \includegraphics[width=0.9\linewidth]{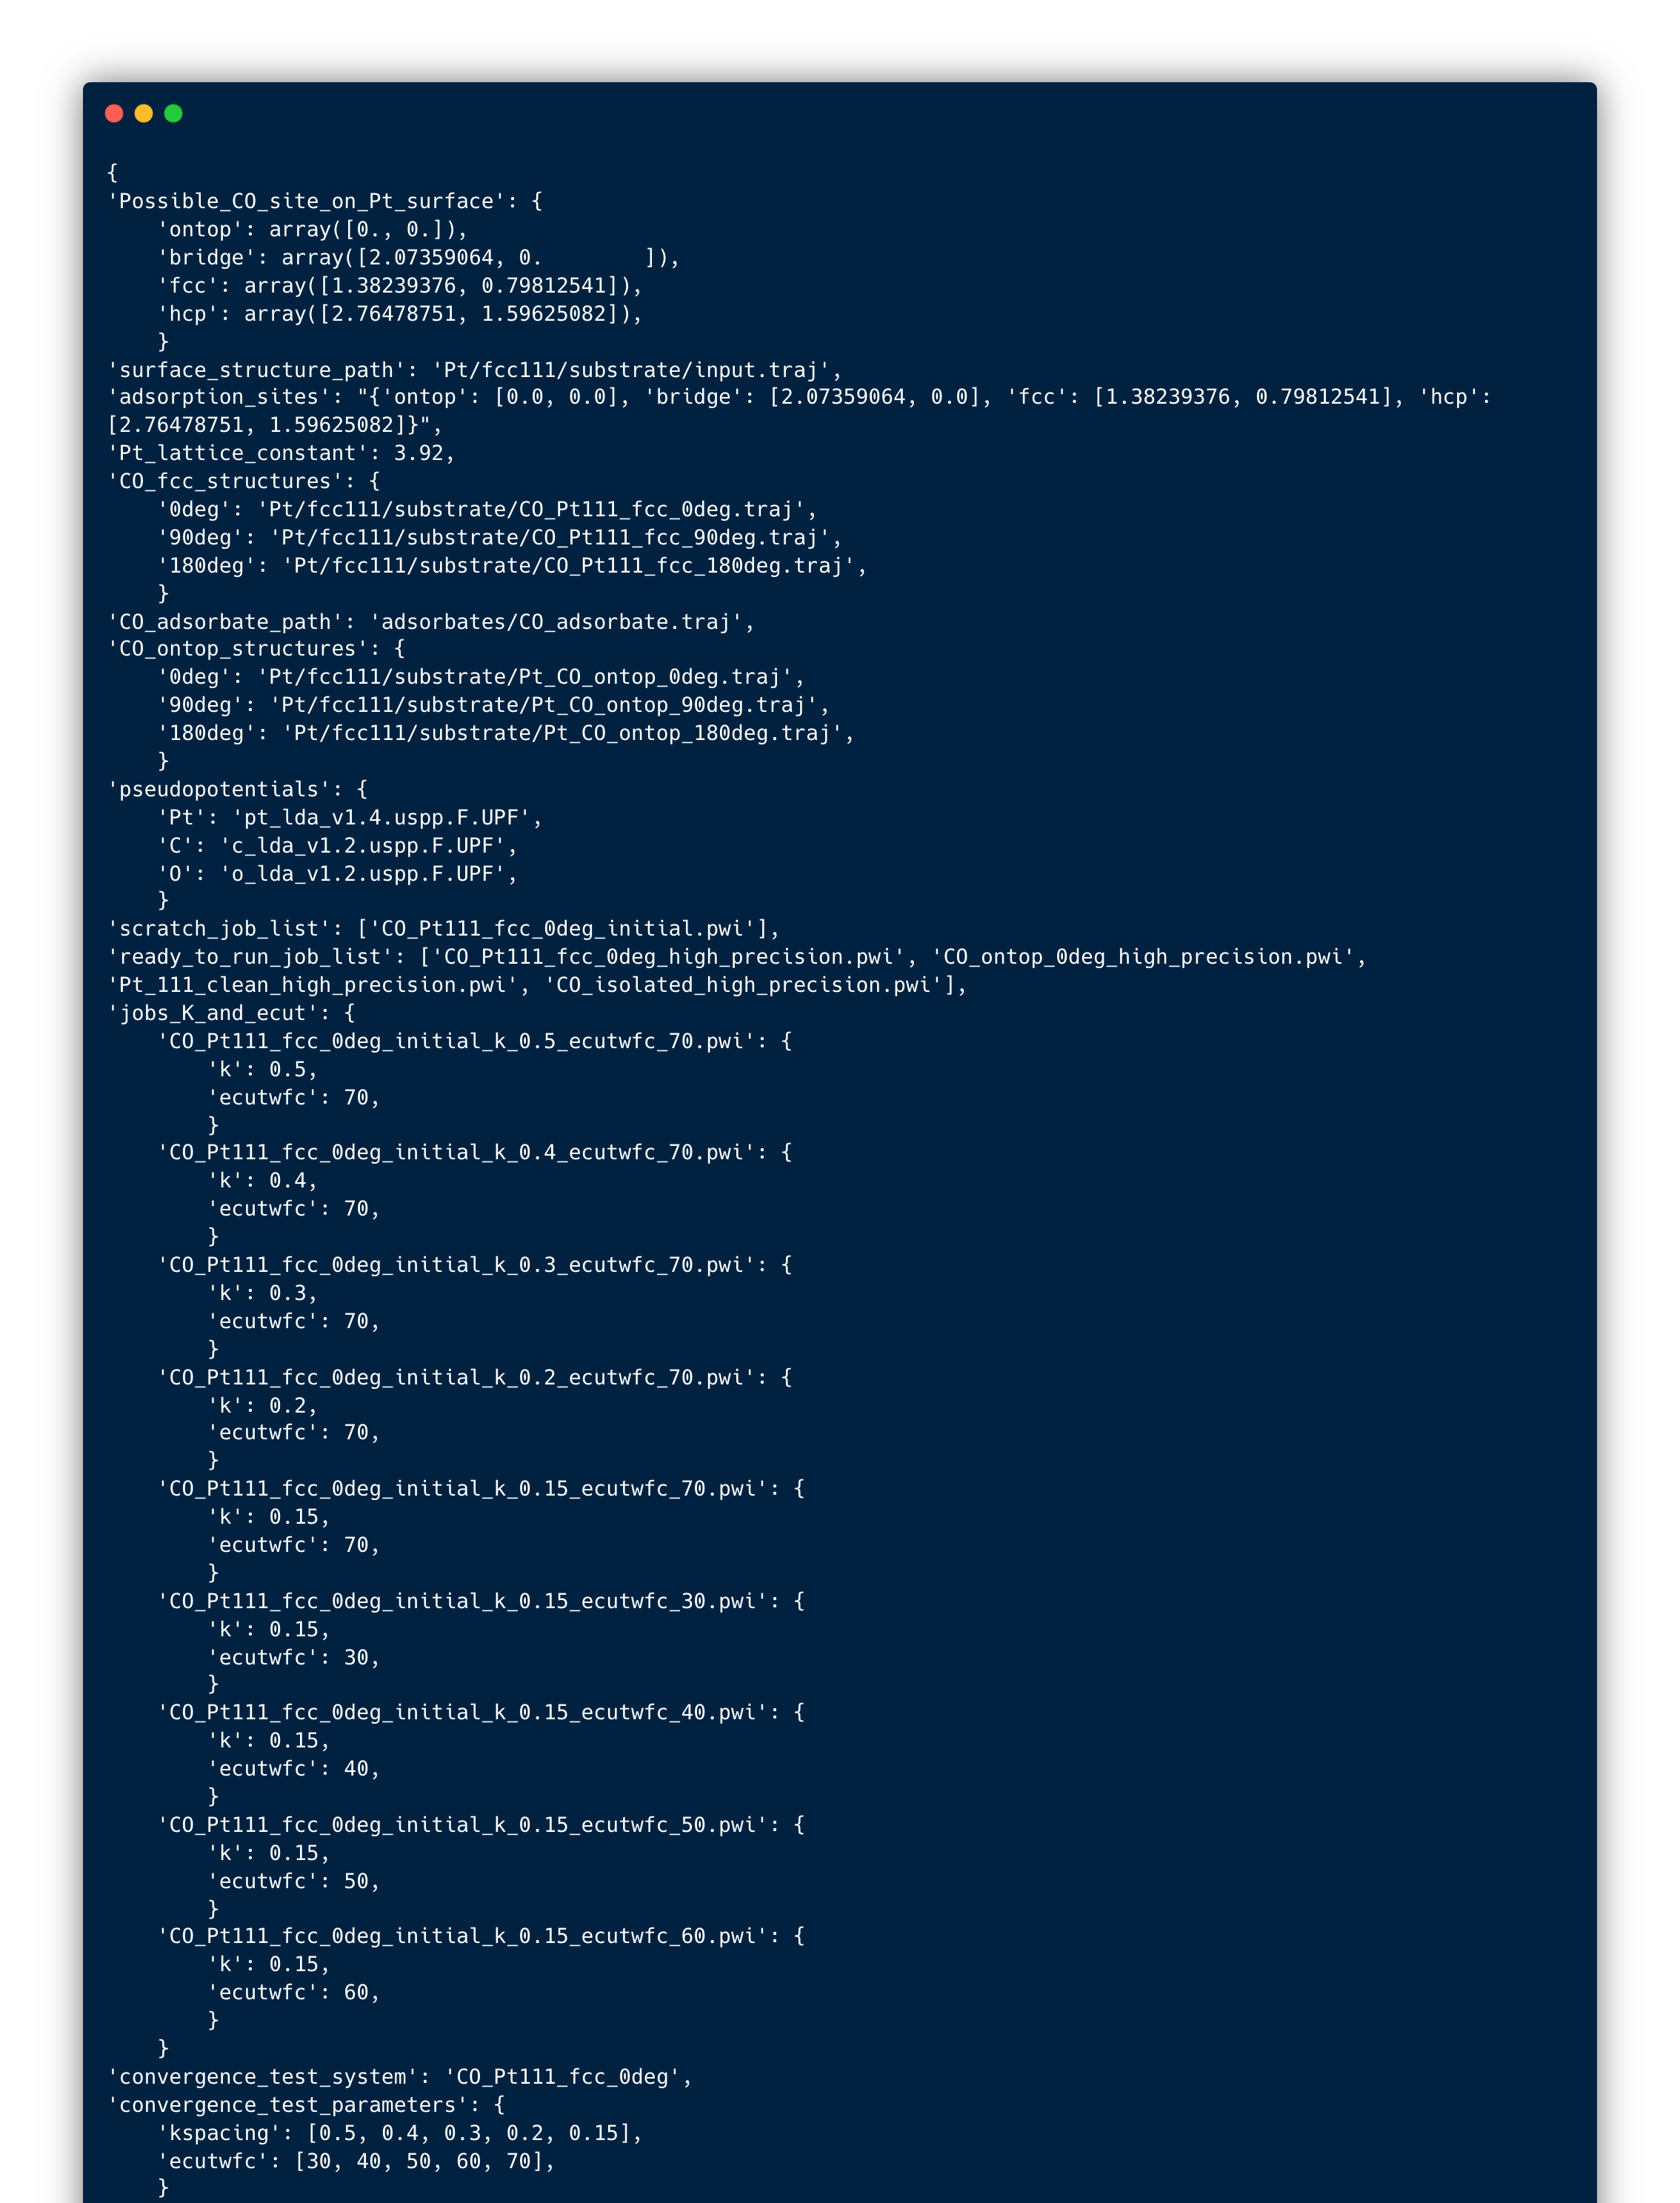}
    \label{fig:enter-label}
\end{figure}

Full Canvas History for CO/Pt(111) Challenge (Cont.)
\begin{figure}[H]
    \centering
    \includegraphics[width=1.0\linewidth]{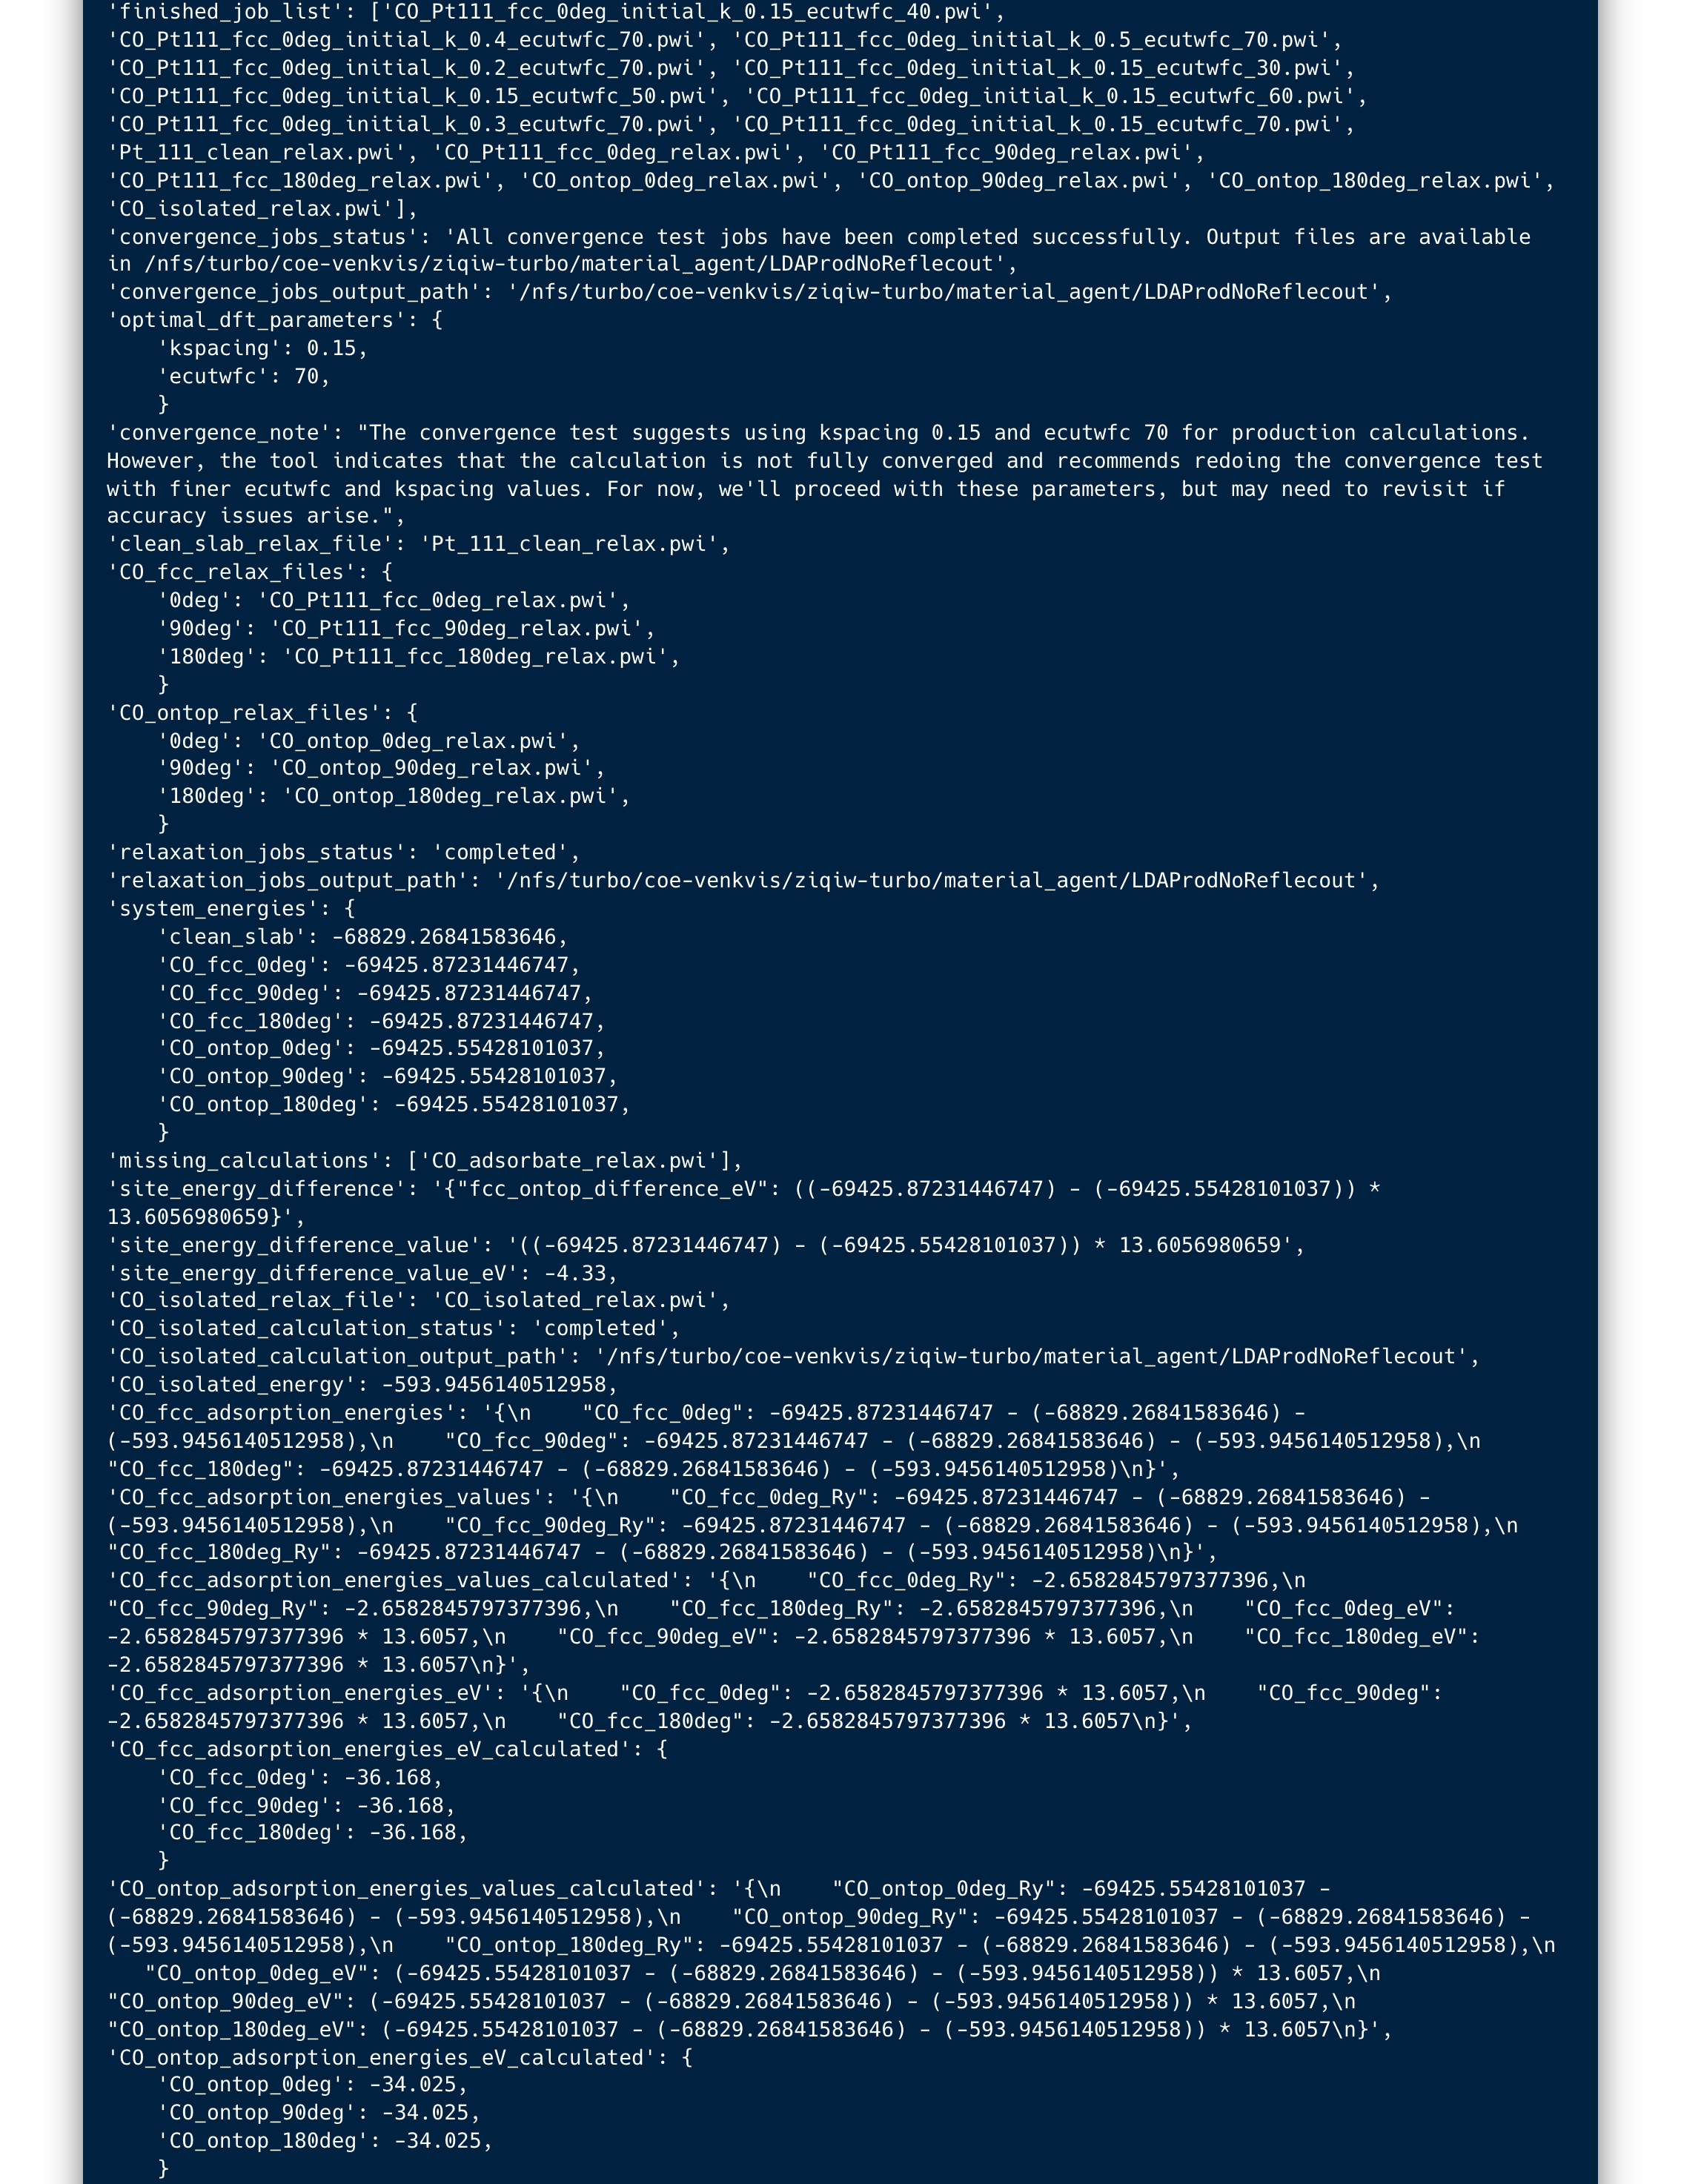}
    \label{fig:enter-label}
\end{figure}

Full Canvas History for CO/Pt(111) Challenge (Cont.)
\begin{figure}[H]
    \centering
    \includegraphics[width=1.0\linewidth]{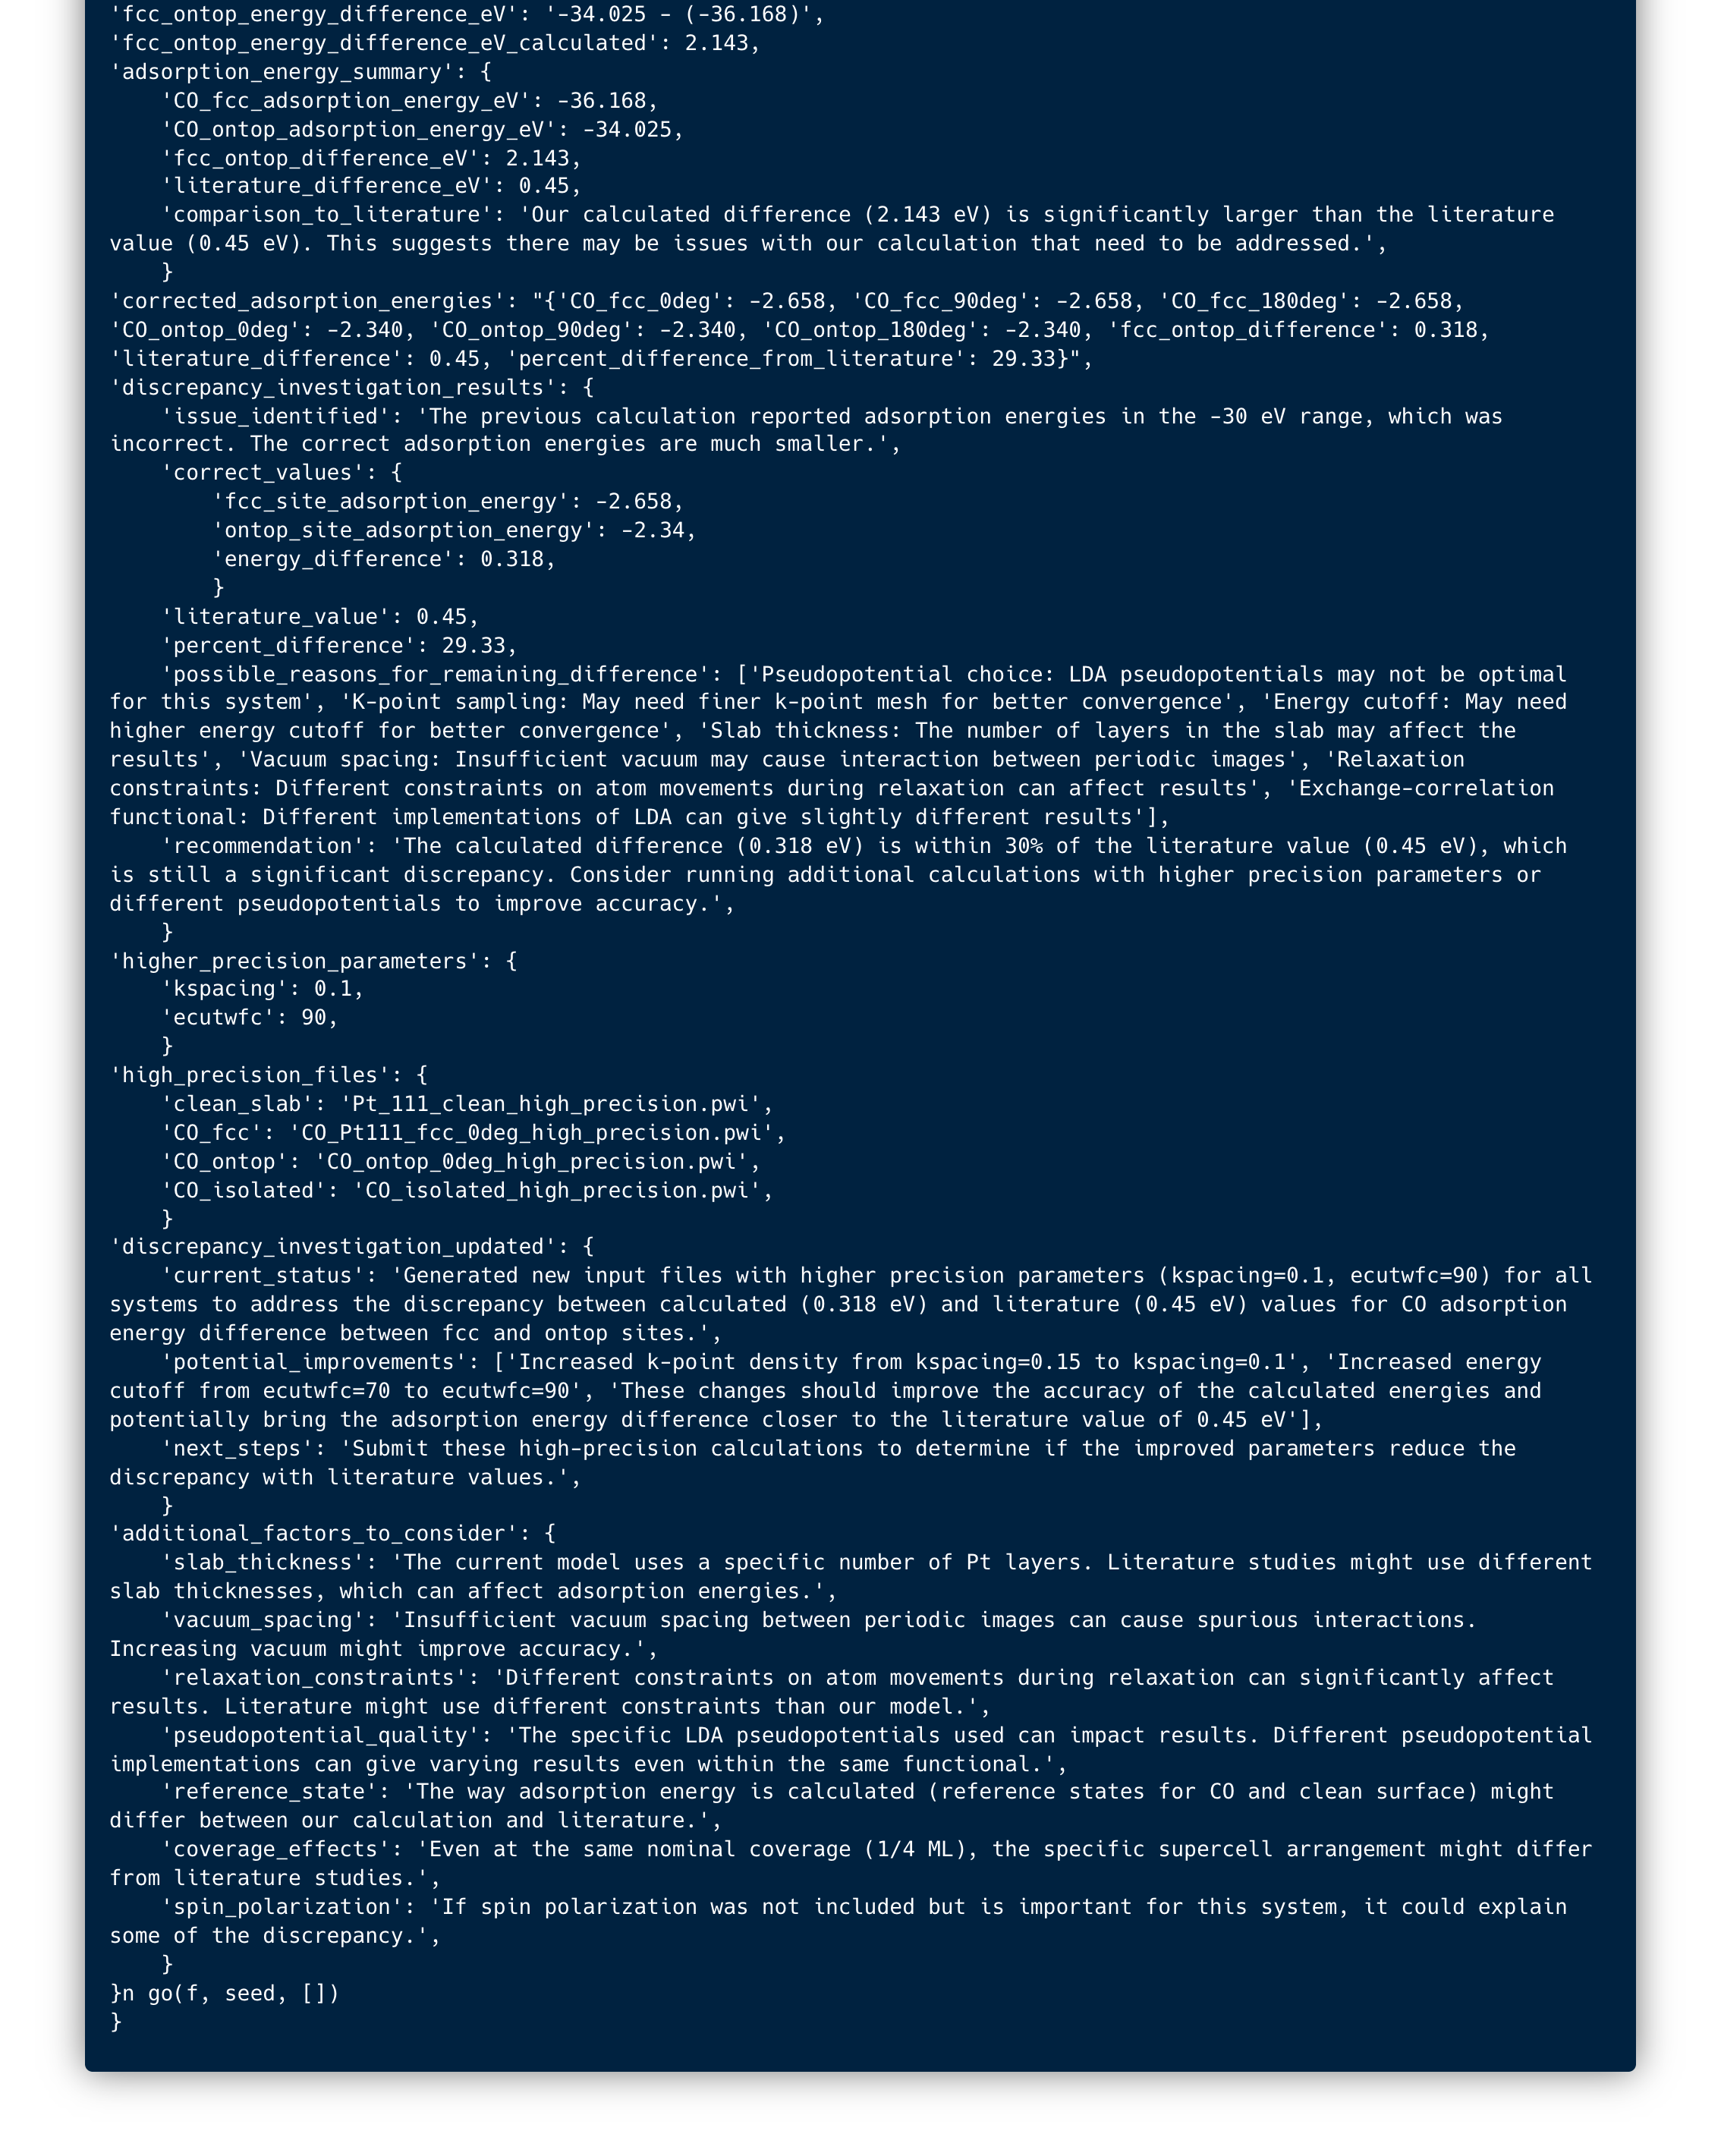}
    \label{fig:enter-label}
\end{figure}

\section*{List of tools provided}
%-------------------------
\paragraph{inspect\_my\_canvas}
\begin{itemize}[leftmargin=2em,label={}, itemsep=0pt, parsep=0pt, topsep=0pt, partopsep=0pt]
  \item \textbf{description:} Inspect the working canvas to get available keys
  \item \textbf{arguments:}
  \begin{itemize}[leftmargin=2em,label={}, itemsep=0pt, parsep=0pt, topsep=0pt, partopsep=0pt]
      \item \textbf{No argument needed}
  \end{itemize}
\end{itemize}

%-------------------------
\paragraph{read\_my\_canvas}
\begin{itemize}[leftmargin=2em,label={}, itemsep=0pt, parsep=0pt, topsep=0pt, partopsep=0pt]
  \item \textbf{description:} Read a value from the working canvas
  \item \textbf{arguments:}
  \begin{itemize}[leftmargin=2em,label={}, itemsep=0pt, parsep=0pt, topsep=0pt, partopsep=0pt]
      \item \textbf{Key}: key
  \end{itemize}
\end{itemize}

%-------------------------
\paragraph{write\_my\_canvas}
\begin{itemize}[leftmargin=2em,label={},itemsep=0pt,parsep=0pt,topsep=0pt,partopsep=0pt]
  \item \textbf{description:} Write a value to the working canvas. If the key already exists, it will not overwrite unless specified.
  \item \textbf{arguments:}
  \begin{itemize}[leftmargin=2em,label={},itemsep=0pt,parsep=0pt,topsep=0pt,partopsep=0pt]
    \item \textbf{key:} key
    \item \textbf{value:} value
    \item \textbf{overwrite:} True to overwrite if key already exist. Only set to True if you are certain you want to overwrite the existing value. (default False)
  \end{itemize}
\end{itemize}

%-------------------------
\paragraph{init\_structure\_data}
\begin{itemize}[leftmargin=2em,label={},itemsep=0pt,parsep=0pt,topsep=0pt,partopsep=0pt]
  \item \textbf{description:} Create single-element bulk initial structure based on crystal lattice and lattice constants, save to working directory, and return filename.
  \item \textbf{arguments:}
  \begin{itemize}[leftmargin=2em,label={},itemsep=0pt,parsep=0pt,topsep=0pt,partopsep=0pt]
    \item \textbf{element:} Element symbol (str)
    \item \textbf{lattice:} Lattice type (str). One of \texttt{sc, fcc, bcc, tetragonal, bct, hcp, rhombohedral, orthorhombic, mcl, diamond, zincblende, rocksalt, cesiumchloride, fluorite, wurtzite}.
    \item \textbf{a:} Lattice constant \(a\) (float)
    \item \textbf{b:} Lattice constant \(b\) (float). If only \(a\) and \(b\) given, \(b\) will be interpreted as \(c\). (default None)
    \item \textbf{c:} Lattice constant \(c\) (float). (default None)
  \end{itemize}
\end{itemize}

%-------------------------
\paragraph{generateSurface\_and\_getPossibleSite}
\begin{itemize}[leftmargin=2em,label={},itemsep=0pt,parsep=0pt,topsep=0pt,partopsep=0pt]
  \item \textbf{description:} Generate a surface structure and return available adsorption sites.
  \item \textbf{arguments:}
  \begin{itemize}[leftmargin=2em,label={},itemsep=0pt,parsep=0pt,topsep=0pt,partopsep=0pt]
    \item \textbf{species:} Element symbol (str)
    \item \textbf{crystal\_structures:} Crystal structure (str). Same options as \texttt{init\_structure\_data}.
    \item \textbf{a\_dict:} Dict of lattice parameters per species, e.g.\ \{\texttt{'Pt':4.0}\}
    \item \textbf{facets:} Facet of the surface (str), e.g.\ \texttt{100,111,…}
    \item \textbf{supercell\_dim:} Supercell repetitions [int,int,int], typically \texttt{[int,int,6]}
    \item \textbf{n\_fixed\_layers:} Number of fixed layers (int), typically 3. (default 3)
  \end{itemize}
\end{itemize}

%-------------------------
\paragraph{generate\_myAdsorbate}
\begin{itemize}[leftmargin=2em,label={},itemsep=0pt,parsep=0pt,topsep=0pt,partopsep=0pt]
  \item \textbf{description:} Generate an adsorbate structure and save it.
  \item \textbf{arguments:}
  \begin{itemize}[leftmargin=2em,label={},itemsep=0pt,parsep=0pt,topsep=0pt,partopsep=0pt]
    \item \textbf{symbols:} Element symbols of the adsorbate (no delimiters) (str)
    \item \textbf{positions:} Atom positions \(\bigl[[x_1,y_1,z_1],…\bigr]\) (list of float triplets)
    \item \textbf{AdsorbateFileName:} File name (not path) ending in \texttt{.traj} (str)
  \end{itemize}
\end{itemize}

%-------------------------
\paragraph{add\_myAdsorbate}
\begin{itemize}[leftmargin=2em,label={},itemsep=0pt,parsep=0pt,topsep=0pt,partopsep=0pt]
  \item \textbf{description:} Add adsorbate(s) to a surface structure and save it.
  \item \textbf{arguments:}
  \begin{itemize}[leftmargin=2em,label={},itemsep=0pt,parsep=0pt,topsep=0pt,partopsep=0pt]
    \item \textbf{mySurfacePath:} Path to surface structure (str)
    \item \textbf{adsorbatePath:} Path to adsorbate structure (str)
    \item \textbf{mySites:} List of 2D site coordinates \(\bigl[[x_1,y_1],…\bigr]\) (list of float pairs)
    \item \textbf{rotations:} List of rotations \(\bigl[[\theta,\text{axis}],…\bigr]\) (list of [float,str])
    \item \textbf{surfaceWithAdsorbateFileName:} Output file name ending in \texttt{.traj} (str)
  \end{itemize}
\end{itemize}

%-------------------------
\paragraph{write\_QE\_script\_w\_ASE}
\begin{itemize}[leftmargin=2em,label={},itemsep=0pt,parsep=0pt,topsep=0pt,partopsep=0pt]
  \item \textbf{description:} Write a Quantum Espresso input using ASE. Bool values unquoted; smearing starts with \texttt{methfessel-paxton}; choose \(\mathtt{ecutwfc}\) 30–100 Ry; ensemble jobs require \texttt{calculation='ensemble'}.
  \item \textbf{arguments:}
  \begin{itemize}[leftmargin=2em,label={},itemsep=0pt,parsep=0pt,topsep=0pt,partopsep=0pt]
    \item \textbf{listofElements:} List of element symbols (list of str)
    \item \textbf{ppfiles:} Pseudopotential filenames in element order (list of str)
    \item \textbf{filename:} Output input file name ending in \texttt{.pwi} (str)
    \item \textbf{inputAtomsDir:} Atoms file dir or job name (str)
    \item \textbf{ensembleCalculation:} Ensemble calculation? (bool)
    \item \textbf{calculation:} \texttt{'scf','relax','ensemble'} (str)
    \item \textbf{restart\_mode:} \texttt{'from\_scratch','restart'} (str)
    \item \textbf{prefix:} Output prefix (str)
    \item \textbf{disk\_io:} \texttt{'none','minimal','nowf','low','medium','high'} (str)
    \item \textbf{ibrav:} Bravais index (int)
    \item \textbf{nat:} Number of atoms (int)
    \item \textbf{ntyp:} Number of types (int)
    \item \textbf{ecutwfc:} Wavefunction cutoff (Ry) (float)
    \item \textbf{ecutrho:} Charge density cutoff (Ry) (float)
    \item \textbf{occupations:} \texttt{'smearing',…} (str)
    \item \textbf{smearing:} \texttt{'gaussian','methfessel-paxton',…} (str)
    \item \textbf{degauss:} Gaussian spread (Ry) (float)
    \item \textbf{conv\_thr:} SCF convergence threshold (float)
    \item \textbf{electron\_maxstep:} Max SCF iterations (int)
    \item \textbf{kspacing:} K-point spacing (\r{A}$^{-1}$) (float)
    \item \textbf{input\_dft:} \texttt{'LDA','PBE','BEEF-vdW'} (str)
    \item \textbf{ready\_to\_run\_job:} Ready to run? (bool) (default False)
    \item \textbf{additional\_input:} Flat dict of extra input parameters (dict) (default \{\})
  \end{itemize}
\end{itemize}

%-------------------------
\paragraph{find\_pseudopotential}
\begin{itemize}[leftmargin=2em,label={},itemsep=0pt,parsep=0pt,topsep=0pt,partopsep=0pt]
  \item \textbf{description:} Return pseudopotential file path for a given element symbol.
  \item \textbf{arguments:}
  \begin{itemize}[leftmargin=2em,label={},itemsep=0pt,parsep=0pt,topsep=0pt,partopsep=0pt]
    \item \textbf{element:} Element symbol (str)
  \end{itemize}
\end{itemize}

%-------------------------
\paragraph{generate\_convergence\_test}
\begin{itemize}[leftmargin=2em,label={},itemsep=0pt,parsep=0pt,topsep=0pt,partopsep=0pt]
  \item \textbf{description:} Generate convergence-test QE input scripts from a template and save job list.
  \item \textbf{arguments:}
  \begin{itemize}[leftmargin=2em,label={},itemsep=0pt,parsep=0pt,topsep=0pt,partopsep=0pt]
    \item \textbf{input\_file\_name:} Template .pwi filename (str)
    \item \textbf{kspacing:} List of k-spacings to test (list of float)
    \item \textbf{ecutwfc:} List of ecutwfc values to test (list of int)
  \end{itemize}
\end{itemize}

%-------------------------
\paragraph{generate\_eos\_test}
\begin{itemize}[leftmargin=2em,label={},itemsep=0pt,parsep=0pt,topsep=0pt,partopsep=0pt]
  \item \textbf{description:} Generate EOS test QE input scripts and save job list.
  \item \textbf{arguments:}
  \begin{itemize}[leftmargin=2em,label={},itemsep=0pt,parsep=0pt,topsep=0pt,partopsep=0pt]
    \item \textbf{input\_file\_name:} Template .pwi filename (str)
    \item \textbf{kspacing:} K-spacing to test (float)
    \item \textbf{ecutwfc:} Ecutwfc to test (int)
    \item \textbf{stepSize:} Scale-step for EOS (float, 0.01–0.1) (default 0.025)
  \end{itemize}
\end{itemize}

%-------------------------
\paragraph{get\_convergence\_suggestions}
\begin{itemize}[leftmargin=2em,label={},itemsep=0pt,parsep=0pt,topsep=0pt,partopsep=0pt]
  \item \textbf{description:} Get DFT convergence suggestions based on output files.
  \item \textbf{arguments:}
  \begin{itemize}[leftmargin=2em,label={},itemsep=0pt,parsep=0pt,topsep=0pt,partopsep=0pt]
    \item \textbf{filename:} Output .pwi filename (str)
    \item \textbf{question:} Query about convergence or accuracy (str)
  \end{itemize}
\end{itemize}

%-------------------------
\paragraph{calculate\_formation\_E}
\begin{itemize}[leftmargin=2em,label={},itemsep=0pt,parsep=0pt,topsep=0pt,partopsep=0pt]
  \item \textbf{description:} Calculate formation energy of an adsorbate on a slab.
  \item \textbf{arguments:}
  \begin{itemize}[leftmargin=2em,label={},itemsep=0pt,parsep=0pt,topsep=0pt,partopsep=0pt]
    \item \textbf{slabFilePath:} Slab .pwi filename (str)
    \item \textbf{adsorbateFilePath:} Adsorbate .pwi filename (str)
    \item \textbf{systemFilePath:} Slab+adsorbate .pwi filename (str)
  \end{itemize}
\end{itemize}

%-------------------------
\paragraph{calculate\_lc}
\begin{itemize}[leftmargin=2em,label={},itemsep=0pt,parsep=0pt,topsep=0pt,partopsep=0pt]
  \item \textbf{description:} Read EOS outputs and calculate lattice constant.
  \item \textbf{arguments:}
  \begin{itemize}[leftmargin=2em,label={},itemsep=0pt,parsep=0pt,topsep=0pt,partopsep=0pt]
    \item \textbf{jobFileIdx:} Indices of finished EOS jobs (list of int)
  \end{itemize}
\end{itemize}

%-------------------------
\paragraph{get\_bulk\_modulus}
\begin{itemize}[leftmargin=2em,label={},itemsep=0pt,parsep=0pt,topsep=0pt,partopsep=0pt]
  \item \textbf{description:} Calculate bulk modulus from QE input and working directory.
  \item \textbf{arguments:}
  \begin{itemize}[leftmargin=2em,label={},itemsep=0pt,parsep=0pt,topsep=0pt,partopsep=0pt]
    \item \textbf{working\_directory:} QE working directory (str)
    \item \textbf{pseudo\_dir:} Pseudopotential directory (str)
    \item \textbf{input\_file:} QE input filename (str)
  \end{itemize}
\end{itemize}

%-------------------------
\paragraph{get\_lattice\_constant}
\begin{itemize}[leftmargin=2em,label={},itemsep=0pt,parsep=0pt,topsep=0pt,partopsep=0pt]
  \item \textbf{description:} Calculate lattice constant from QE input and working directory.
  \item \textbf{arguments:}
  \begin{itemize}[leftmargin=2em,label={},itemsep=0pt,parsep=0pt,topsep=0pt,partopsep=0pt]
    \item \textbf{working\_directory:} QE working directory (str)
    \item \textbf{pseudo\_dir:} Pseudopotential directory (str)
    \item \textbf{input\_file:} QE input filename (str)
  \end{itemize}
\end{itemize}

%-------------------------
\paragraph{get\_kspacing\_ecutwfc}
\begin{itemize}[leftmargin=2em,label={},itemsep=0pt,parsep=0pt,topsep=0pt,partopsep=0pt]
  \item \textbf{description:} Determine optimal k-spacing and ecutwfc from convergence tests.
  \item \textbf{arguments:}
  \begin{itemize}[leftmargin=2em,label={},itemsep=0pt,parsep=0pt,topsep=0pt,partopsep=0pt]
    \item \textbf{jobFileIdx:} Indices of convergence jobs (list of int)
    \item \textbf{threshold:} Energy threshold (meV/atom) (float, default 1.0)
  \end{itemize}
\end{itemize}

%-------------------------
\paragraph{analyze\_BEEF\_result}
\begin{itemize}[leftmargin=2em,label={},itemsep=0pt,parsep=0pt,topsep=0pt,partopsep=0pt]
  \item \textbf{description:} Read BEEF ensemble outputs, compute adsorption energies, and analyze results.
  \item \textbf{arguments:}
  \begin{itemize}[leftmargin=2em,label={},itemsep=0pt,parsep=0pt,topsep=0pt,partopsep=0pt]
    \item \textbf{slabFilePath:} Clean slab .pwi filename (str)
    \item \textbf{adsorbateFilePath:} Adsorbate .pwi filename (str)
    \item \textbf{ontopFilePath:} Ontop adsorbate .pwi filename (str)
    \item \textbf{fccFilePath:} FCC adsorbate .pwi filename (str)
  \end{itemize}
\end{itemize}

%-------------------------
\paragraph{add\_resource\_suggestion}
\begin{itemize}[leftmargin=2em,label={},itemsep=0pt,parsep=0pt,topsep=0pt,partopsep=0pt]
  \item \textbf{description:} Save DFT resource suggestions and submission script in the working directory.
  \item \textbf{arguments:}
  \begin{itemize}[leftmargin=2em,label={},itemsep=0pt,parsep=0pt,topsep=0pt,partopsep=0pt]
    \item \textbf{qeInputFileName:} DFT input filename (str)
    \item \textbf{partition:} SLURM partition (str)
    \item \textbf{nnodes:} Number of nodes (int)
    \item \textbf{ntasks:} Number of tasks (int)
    \item \textbf{runtime:} Time limit in minutes (str)
    \item \textbf{submissionScript:} Submission script (no \#SBATCH) (str)
    \item \textbf{outputFilename:} Output filename (str)
  \end{itemize}
\end{itemize}

%-------------------------
\paragraph{submit\_and\_monitor\_job}
\begin{itemize}[leftmargin=2em,label={},itemsep=0pt,parsep=0pt,topsep=0pt,partopsep=0pt]
  \item \textbf{description:} Submit and monitor jobs using saved resource suggestions.
  \item \textbf{arguments:}
  \begin{itemize}[leftmargin=2em,label={},itemsep=0pt,parsep=0pt,topsep=0pt,partopsep=0pt]
    \item \textbf{jobType:} Type of job, e.g.\ \texttt{'DFT','LAMMPS'} (str)
  \end{itemize}
\end{itemize}

%-------------------------
\paragraph{read\_energy\_from\_output}
\begin{itemize}[leftmargin=2em,label={},itemsep=0pt,parsep=0pt,topsep=0pt,partopsep=0pt]
  \item \textbf{description:} Read total energy from finished job outputs.
  \item \textbf{arguments:}
  \begin{itemize}[leftmargin=2em,label={},itemsep=0pt,parsep=0pt,topsep=0pt,partopsep=0pt]
    \item \textbf{jobFileIdx:} Indices of finished jobs (list of int)
  \end{itemize}
\end{itemize}

\includepdf[
  pagecommand=\section{CO/Pt(111) Full log: structure preparation},
  pages=1-12,       % which pages of the PDF to include
  nup=4x4,         % arrange them in 2 columns × 2 rows
  frame=true,      % draw a frame around each panel
  delta=5mm 5mm,   % horizontal and vertical gap between panels
  offset= 0mm -30mm,
  scale=0.9      % (optional) scale each panel slightly
]{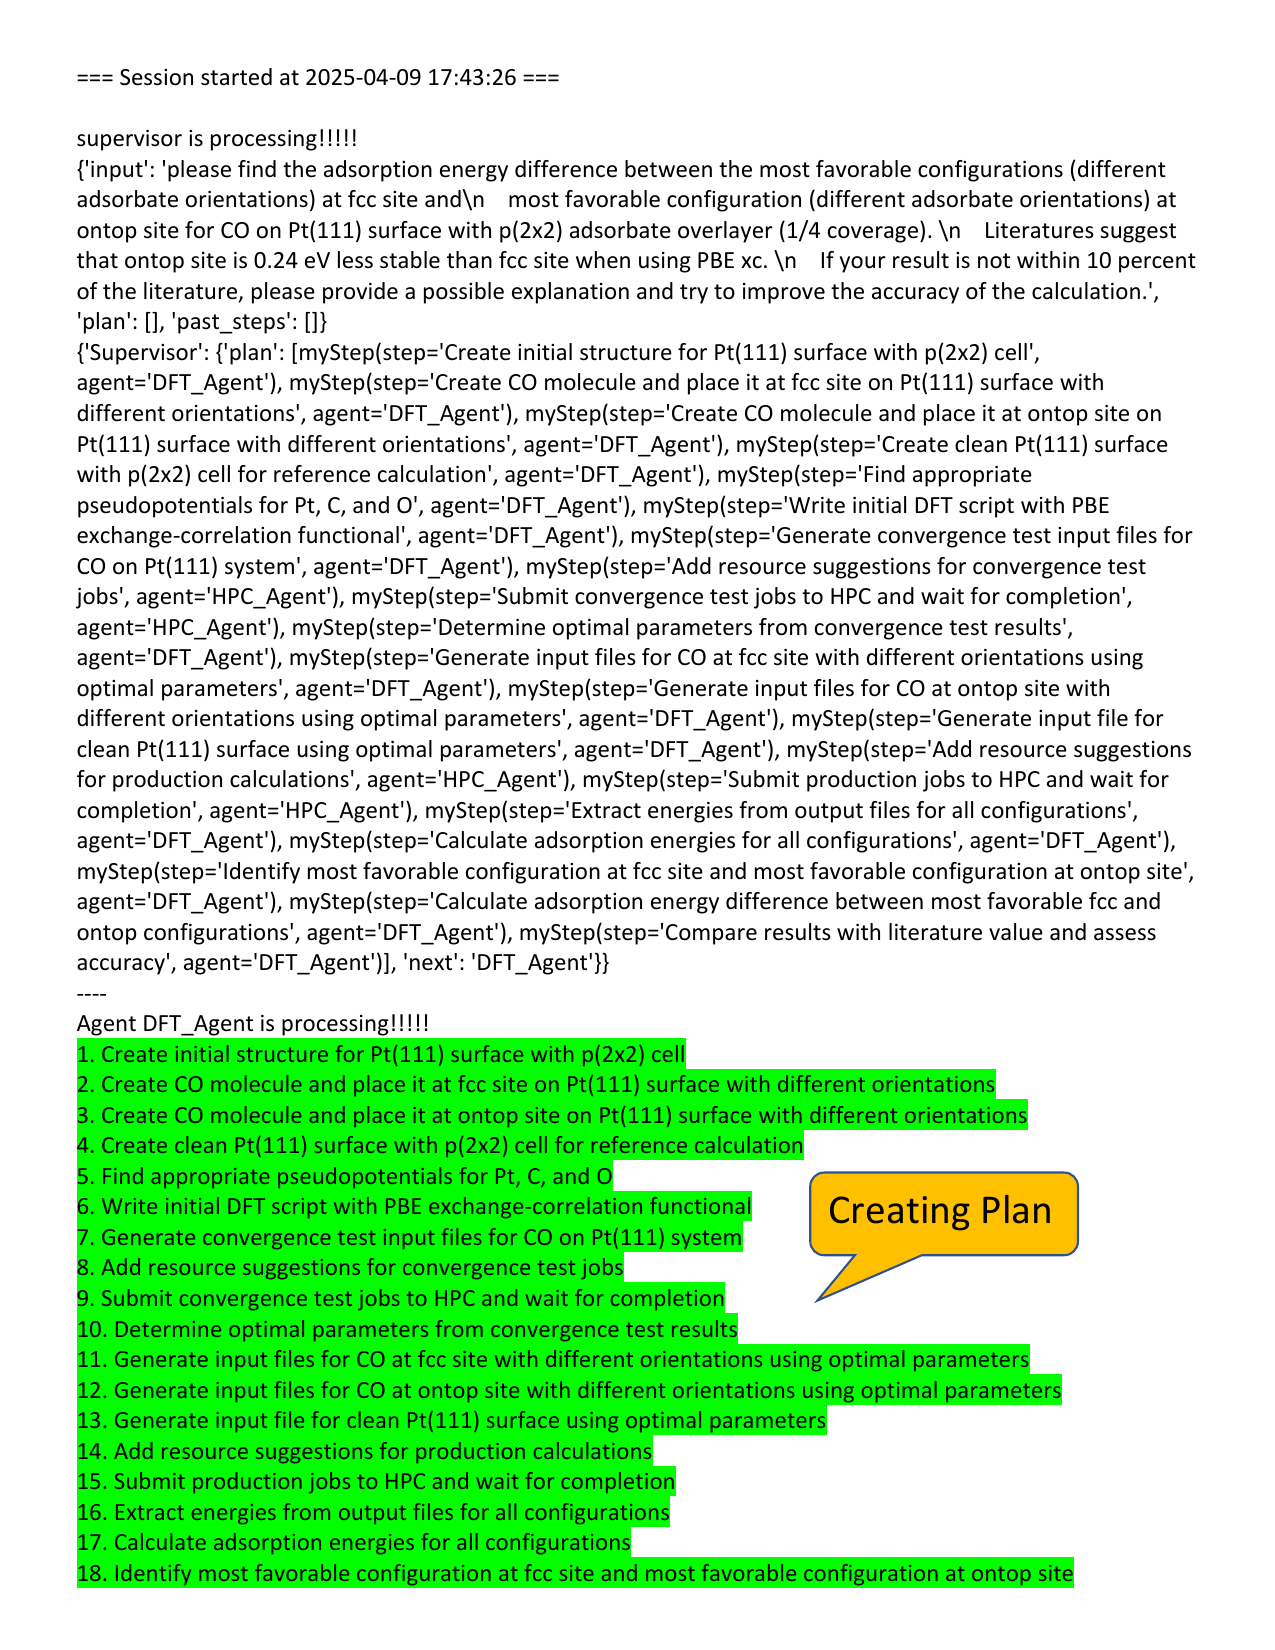}

\includepdf[
  pagecommand=\section{CO/Pt(111) Full log: DFT script generation},
  pages=13-24,       % which pages of the PDF to include
  nup=4x4,         % arrange them in 2 columns × 2 rows
  frame=true,      % draw a frame around each panel
  delta=5mm 5mm,   % horizontal and vertical gap between panels
  offset= 0mm -30mm,
  scale=0.9      % (optional) scale each panel slightly
]{pdfs/gen2coptdemoForPaper.pdf}

\includepdf[
  pagecommand=\section{CO/Pt(111) Full log: convergence test generation},
  pages=25-27,       % which pages of the PDF to include
  nup=2x3,         % arrange them in 2 columns × 2 rows
  frame=true,      % draw a frame around each panel
  delta=5mm 5mm,   % horizontal and vertical gap between panels
  offset= 0mm -30mm,
  scale=0.9      % (optional) scale each panel slightly
]{pdfs/gen2coptdemoForPaper.pdf}

\includepdf[
  pagecommand=\section{CO/Pt(111) Full log: HPC job submission and monitor},
  pages=28-34,       % which pages of the PDF to include
  nup=4x3,         % arrange them in 2 columns × 2 rows
  frame=true,      % draw a frame around each panel
  delta=5mm 5mm,   % horizontal and vertical gap between panels
  offset= 0mm -30mm,
  scale=0.9      % (optional) scale each panel slightly
]{pdfs/gen2coptdemoForPaper.pdf}

\includepdf[
  pagecommand=\section{CO/Pt(111) Full log: convergence issue handling for convergence test run},
  pages=35-37,       % which pages of the PDF to include
  nup=2x3,         % arrange them in 2 columns × 2 rows
  frame=true,      % draw a frame around each panel
  delta=5mm 5mm,   % horizontal and vertical gap between panels
  offset= 0mm -40mm,
  scale=0.9      % (optional) scale each panel slightly
]{pdfs/gen2coptdemoForPaper.pdf}

\includepdf[
  pagecommand=\section{CO/Pt(111) Full log: production script generation},
  pages=38-41,       % which pages of the PDF to include
  nup=2x3,         % arrange them in 2 columns × 2 rows
  frame=true,      % draw a frame around each panel
  delta=5mm 5mm,   % horizontal and vertical gap between panels
  offset= 0mm -30mm,
  scale=0.9      % (optional) scale each panel slightly
]{pdfs/gen2coptdemoForPaper.pdf}

\includepdf[
  pagecommand=\section{CO/Pt(111) Full log: handling missed CO script},
  pages=42-46,       % which pages of the PDF to include
  nup=3x3,         % arrange them in 2 columns × 2 rows
  frame=true,      % draw a frame around each panel
  delta=5mm 5mm,   % horizontal and vertical gap between panels
  offset= 0mm -30mm,
  scale=0.9      % (optional) scale each panel slightly
]{pdfs/gen2coptdemoForPaper.pdf}

\includepdf[
  pagecommand=\section{CO/Pt(111) Full log: handling first convergence issue for production run},
  pages=47-56,       % which pages of the PDF to include
  nup=4x4,         % arrange them in 2 columns × 2 rows
  frame=true,      % draw a frame around each panel
  delta=5mm 5mm,   % horizontal and vertical gap between panels
  offset= 0mm -40mm,
  scale=0.9      % (optional) scale each panel slightly
]{pdfs/gen2coptdemoForPaper.pdf}

\includepdf[
  pagecommand=\section{CO/Pt(111) Full log: handling second convergence issue for production run},
  pages=57-67,       % which pages of the PDF to include
  nup=4x4,         % arrange them in 2 columns × 2 rows
  frame=true,      % draw a frame around each panel
  delta=5mm 5mm,   % horizontal and vertical gap between panels
  offset= 0mm -40mm,
  scale=0.9      % (optional) scale each panel slightly
]{pdfs/gen2coptdemoForPaper.pdf}

\includepdf[
  pagecommand=\section{CO/Pt(111) Full log: post-processing},
  pages=68-71,       % which pages of the PDF to include
  nup=2x3,         % arrange them in 2 columns × 2 rows
  frame=true,      % draw a frame around each panel
  delta=5mm 5mm,   % horizontal and vertical gap between panels
  offset= 0mm -40mm,
  scale=0.9      % (optional) scale each panel slightly
]{pdfs/gen2coptdemoForPaper.pdf}

% \begin{Verbatim}[breaklines=true, breakanywhere=true]
% {\fontsize{10pt}{6pt}\selectfont

% \end{Verbatim}

%%%%%%%%%%%%%%%%%%%%%%%%%%%%%%%%%%%%%%%%%%%%%%%%%%%%%%%%%%%%%%%%%%%%%
%% The same is true for Supporting Information, which should use the
%% suppinfo environment.
%%%%%%%%%%%%%%%%%%%%%%%%%%%%%%%%%%%%%%%%%%%%%%%%%%%%%%%%%%%%%%%%%%%%%
% \begin{suppinfo}

% This will usually read something like: ``Experimental procedures and
% characterization data for all new compounds. The class will
% automatically add a sentence pointing to the information on-line:

% \end{suppinfo}

%%%%%%%%%%%%%%%%%%%%%%%%%%%%%%%%%%%%%%%%%%%%%%%%%%%%%%%%%%%%%%%%%%%%%
%% The appropriate \bibliography command should be placed here.
%% Notice that the class file automatically sets \bibliographystyle
%% and also names the section correctly.
%%%%%%%%%%%%%%%%%%%%%%%%%%%%%%%%%%%%%%%%%%%%%%%%%%%%%%%%%%%%%%%%%%%%%
% \bibliography{sample}

\end{document}
